# Supplementary material for: Regression for spherical responses with linear and spherical covariates using a scaled link function
Source: arXiv:2509.06204 ancillary file (2025-09-07)
Supplement: Supplementary file 1 [file reproduce_midatlantic.pdf]

# Mid-Atlantic Regression

## Table of contents

|           |                                            |          |
|-----------|--------------------------------------------|----------|
| <b>1</b>  | <b>Data</b>                                | <b>2</b> |
| <b>2</b>  | <b>Euc Covariates</b>                      | <b>2</b> |
| <b>3</b>  | <b>Our SvMF Model</b>                      | <b>2</b> |
| <b>4</b>  | <b>Pretty Data Plot</b>                    | <b>2</b> |
| <b>5</b>  | <b>Predictions</b>                         | <b>3</b> |
| 5.1       | Table of Estimates . . . . .               | 5        |
| 5.2       | Plot . . . . .                             | 6        |
| <b>6</b>  | <b>LOOCV MSE</b>                           | <b>7</b> |
| <b>7</b>  | <b>Residual Size</b>                       | <b>8</b> |
| <b>8</b>  | <b>DoF</b>                                 | <b>8</b> |
| <b>9</b>  | <b>AIC</b>                                 | <b>8</b> |
| <b>10</b> | <b>Main Figure</b>                         | <b>9</b> |
| <b>11</b> | <b>Appendix</b>                            | <b>9</b> |
| 11.1      | Hessian of Likelihood at Optimum . . . . . | 9        |
| 11.2      | Check Other Starts for vMF . . . . .       | 10       |
| 11.3      | Check Other Starts for SvMF . . . . .      | 11       |

---

Code version: 0.0.17

## 1 Data

## 2 Euc Covariates

```
xe <- fulldf %>%  
  select(westedge)  
xestd <- xe %>% scale() %>% as_tibble()
```

## 3 Our SvMF Model

## 4 Pretty Data Plot

```
ymean <- colMeans(fulldf %>% select(starts_with("Y")))  
ymean <- ymean/sqrt(sum(ymean^2))  
#project to equator  
ymeanproj <- c(ymean[1:2], 0)  
ymeanproj/vnorm(ymeanproj)
```

|  | Y1        | Y2         |
|--|-----------|------------|
|  | 0.8791608 | -0.4765251 |
|  | 0.0000000 |            |

```
target <- c(1,0,0)  
prettyrot <- rotationmat_amaral(ymeanproj, target)  
prettyY <- (fulldf %>%  
  select(Y1, Y2, Y3) %>%  
  as.matrix()) %*% t(prettyrot)  
colnames(prettyY) <- paste0("Y", 1:3)  
prettyX <- (fulldf %>%  
  select(X1, X2, X3) %>%  
  as.matrix()) %*% t(prettyrot)  
colnames(prettyX) <- paste0("X", 1:3)  
prettyXmean <- colMeans(prettyX)  
prettyXmean <- prettyXmean/vnorm(prettyXmean)  
# denomloc <- drop(prettyrot %*% as_mnlink_cann(mod$mean)$Qs[,1])  
plotdata <- bind_cols(prettyY, prettyX, westedge = fulldf$westedge) %>%  
  as_tibble() %>%
```

```

ggplot() +
  geom_segment(aes(x=X2, y=X3, xend=Y2, yend=Y3), lty = "dashed", col = "grey") +
  geom_point(aes(x=Y2, y=Y3), shape = 4) +
  geom_point(aes(x=X2, y=X3, fill = westedge), show.legend = FALSE, shape = 21) +
  geom_path(data = circle_df, aes(x = x, y = y), inherit.aes = FALSE, color = "grey") +
  scale_fill_manual(values = c("black", "white")) +
  theme_void() +
  coord_fixed()
# mark mean of spherical covariate (obtained earlier)
# annotate("point", x = prettyXmean[2], y = prettyXmean[3], shape = 24, size = 2)
# annotate("point", x = denomloc[2], y = denomloc[3], shape = 3, size = 4, col = "blue")
plotdata

```

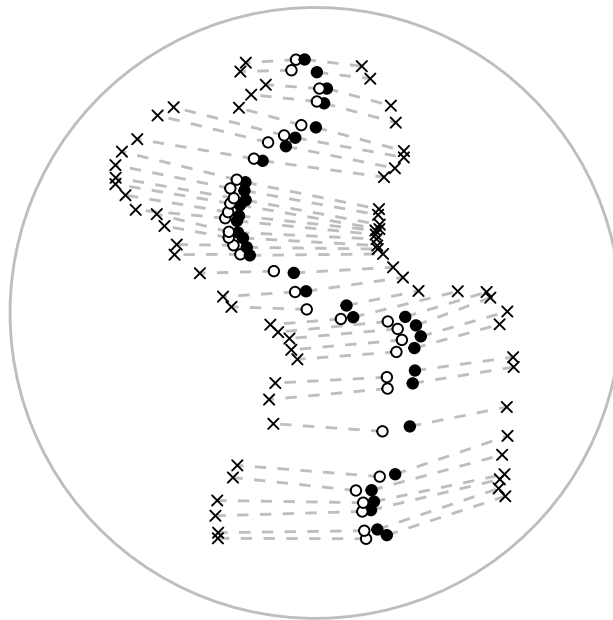

## 5 Predictions

The below ‘ours’ model is using LinEuc’s link with an extra covariate for an intercept and G01 free. The results here are from a local optimisation using gradient from default starting values. I’ve checked that global search for the best vMF regression does not find anything better.

```
cann <- as_mnlink_cann(mod$mean)
cann
```

```
$P
      [,1]      [,2]      [,3]
Y1  0.4913098  0.5626852 -0.66483081
Y2 -0.4803628 -0.4616721 -0.74572812
Y3 -0.7265440  0.6857435  0.04346907
```

```
$Bs
      [,1]      [,2]
[1,] 0.902965 0.0000000
[2,] 0.000000 0.7702707
```

```
$Qs
      [,1]      [,2]      [,3]
X1  0.2657935  0.5868953 -0.7647926
X2 -0.5034122 -0.5920729 -0.6293059
X3 -0.8221496  0.5522713  0.1380811
```

```
$Be
      [,1]      [,2]
[1,] 0.07230433 0.0000000
[2,] 0.00000000 0.2525752
```

```
$Qe
      [,1]      [,2]      [,3]
dummyzero    1  0.0000000 0.0000000
westedge      0  0.1254317 0.9921023
ones          0 -0.9921023 0.1254317
```

```
$ce
[1] 1
```

```
attr("class")
[1] "mnlink_cann" "list"
```

Lets try to interpret the fitted link.

```
cann$Bs %*% t(cann$Qs[,-1])
```

|      | X1         | X2         | X3        |
|------|------------|------------|-----------|
| [1,] | 0.5299459  | -0.5346211 | 0.4986817 |
| [2,] | -0.5890973 | -0.4847359 | 0.1063598 |

```
cann$Be %*% t(cann$Qe[,-1])
```

|      | dummyzero | westedge    | ones        |
|------|-----------|-------------|-------------|
| [1,] | 0         | 0.009069259 | -0.07173329 |
| [2,] | 0         | 0.250580385 | 0.03168094  |

The first direction away from  $B_{01}$  (first row in above) is roughly equally influenced by X1, X2 and X3 (all are about 0.5) with west edge having very little influence (given the values of standardised westedge). The second direction away from  $B_{01}$  (second row in above) is roughly equally influenced by X1 and X2 but much less by X3 (which is the N-S direction) and westedge plays a role.

```
cann$Qs[,1]
```

|  | X1        | X2         | X3         |
|--|-----------|------------|------------|
|  | 0.2657935 | -0.5034122 | -0.8221496 |

Some general scaling occurs with greater influence from X3 (N-S direction), then X2 then X1.

## 5.1 Table of Estimates

```
df <- cbind("diag($B_s$)" = diag(cann$Bs),
            "diag($B_e$)" = diag(cann$Be),
            tQe = t(cann$Qe[,-1])) %>%
  as.data.frame()
row.names(df) <- c("$t_2$", "$t_3$")
mykbl <- kbl(df, booktabs = TRUE, position = "!h", escape = FALSE, format = "latex", digits = 3,
             add_header_above(c(" " = 3, "$R_e^{\top}$" = 2), escape = FALSE))
mykbl
```

|       | diag( $B_s$ ) | diag( $B_e$ ) | $R_e^\top$ |       |
|-------|---------------|---------------|------------|-------|
|       |               |               | westedge   | ones  |
| $t_2$ | 0.90          | 0.07          | 0.13       | -0.99 |
| $t_3$ | 0.77          | 0.25          | 0.99       | 0.13  |

## 5.2 Plot

Note that we have not optimised  $Q$  for ESAG2 because optimisation did not converge.

Ours

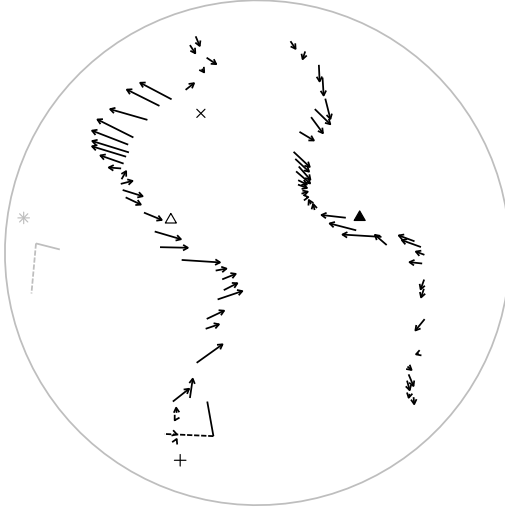

IAG1

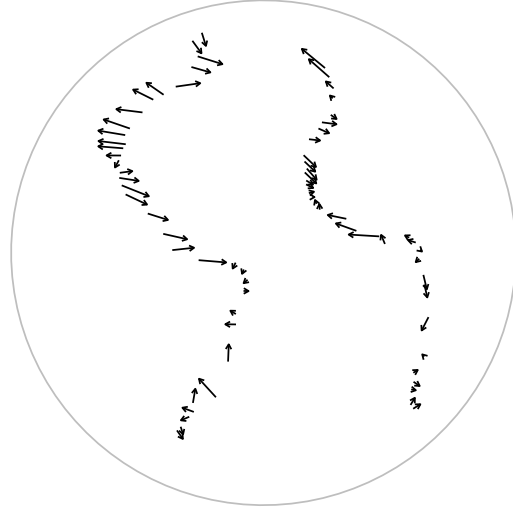

ESAG1

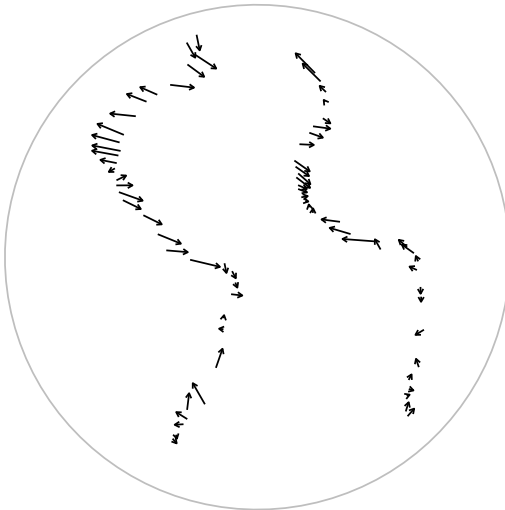

ESAG2

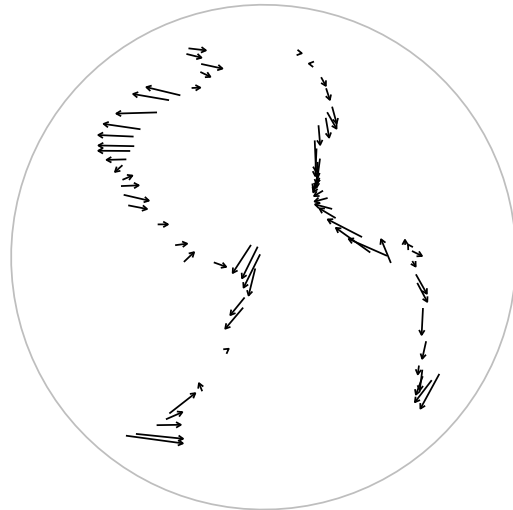

## 6 LOOCV MSE

```
loocvmseSvMF <- function(mod){
  stopifnot(inherits(mod$mean, "mnlink_Omega"))
  dists <- pbapply::pblapply(1:nrow(mod$y), function(idx){
    newmod <- mobius_SvMF(mod$y[-idx,],
      xs = mod$xs[-idx,],
      xe = mod$xe[-idx,c(-1,-ncol(mod$xe)), drop = FALSE],
      fix_qs1 = FALSE,
      type = "LinEuc",
      G01behaviour = "free",
      mean = mod$mean,
      k = mod$k,
      a = mod$a,
      G0 = mod$G0)
    pred <- mnlink(xs = mod$xs[idx,, drop = FALSE],
      xe = mod$xe[idx,, drop = FALSE],
      param = newmod$mean)
    obs <- mod$y[idx,]
    Euc <- vnorm(drop(obs - pred))
    angle <- acos(rowSums(obs * pred))
    return(c(
      Euc = Euc,
      angle = angle
    ))
  })
  dists <- dists %>%
    simplify2array() %>%
    t() %>%
    as_tibble()
  dists %>%
    summarise(across(everything(), ~sum(.x^2)/nrow(mod$y)))
}
loocvmseSvMF(mod)
```

```
# A tibble: 1 x 2
  Euc   angle
<dbl> <dbl>
1 0.0107 0.0107
```

Both of these are smaller than the LOOCV MSE that Rosenthal's PLT achieved of 0.074,

which corresponds to the Euc metric MSE.

## 7 Residual Size

Geodesic distance between predicted mean and observation

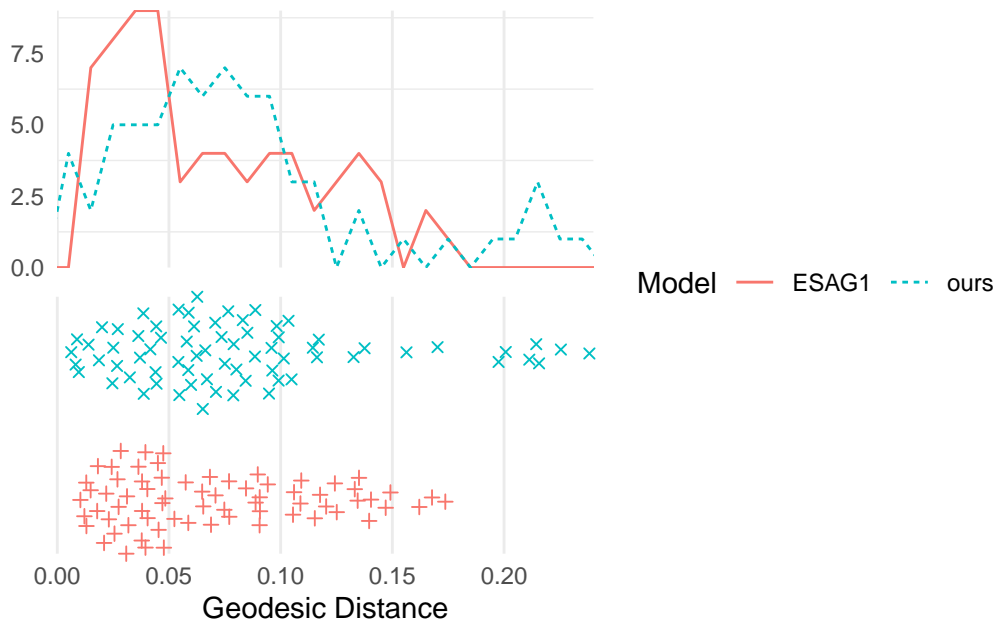

## 8 DoF

| Ours | IAG1 | ESAG1 | ESAG2 |
|------|------|-------|-------|
| 16   | 17   | 22    | 25    |

## 9 AIC

| Ours      | IAG1      | ESAG1     | ESAG2     |
|-----------|-----------|-----------|-----------|
| -463.2407 | -370.7254 | -459.5946 | -436.2852 |



## 10 Main Figure

```
(plotdata + ggtitle("(a) data") + theme(plot.title = element_text(hjust = 0.5))) +
(plotours + theme(legend.position = "none", plot.title = element_text(hjust = 0.5)) + ggtitle(
  (plotESAG1 + ggtitle("(c) structure 1") + theme(plot.title = element_text(hjust = 0.5))) +
  (plotESAG2 + ggtitle("(d) structure 2") + theme(plot.title = element_text(hjust = 0.5))) +
  plot_layout(ncol = 4, widths = c(3,3,3,3))
```

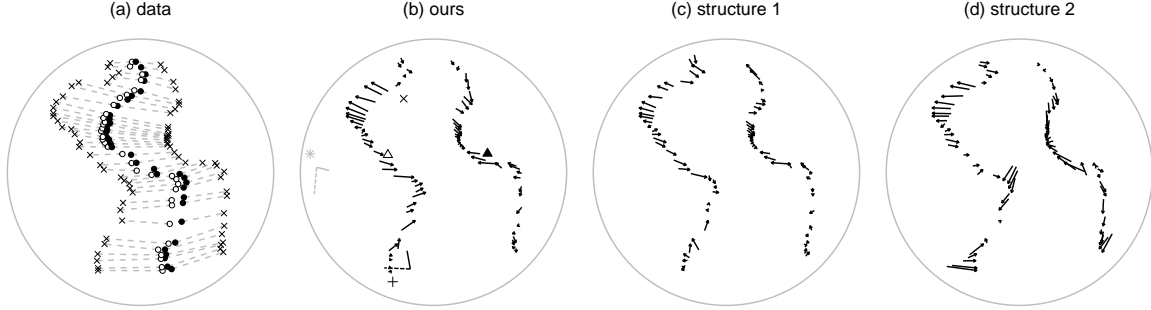

```
ggsave("midatlantic_fig.pdf", width = 12, height = 3.5)
```

Caption: Regression for the midatlantic ridge data. From left: midatlantic ridge (circles) and corresponding locations on the continent (crosses) from Rosenthal et al (2014); our regression; Paine et al structure 1 regression; Paine et al structure 2 regression. The sphere is shown orthogonally projected with north pointing up the page. Arrows: start at the predicted mean and end at the observed continental location, and thus represent residuals. Filled symbols: eastern side. Unfilled symbols: western side. Triangles: Mean of ridge locations and corresponding predicted mean for western or eastern side. Plus symbol: estimated value of  $r_{s1}$ . Pair of black lines: direction of the estimated second (solid) and third (dashed) columns of  $B_0$  located at the estimated first column  $b_{01}$  of  $B_0$ . Pair of grey lines: estimated directions of  $\gamma_{02}$  (solid) and  $\gamma_{03}$  (dashed) located at the estimated  $\gamma_{01}$ .

## 11 Appendix

### 11.1 Hessian of Likelihood at Optimum

The parameter vector is longer than the DoF because of the constraints in the optimisation. There should be  $\text{DoF} + (3-1) * (3 - 2) / 2$  positive eigenvalues. The term  $(3-1) * (3 - 2) / 2$  is for the commutativity constraint on Omega, which the likelihood computation does not account for, so appears as extra degrees of freedom in the Hessian of the likelihood.

```

[1] 8.278212e+03 6.695310e+03 2.997127e+03 2.469711e+03 1.230022e+03
[6] 3.528891e+02 9.513351e+01 2.857011e+01 2.110683e+01 9.720089e+00
[11] 5.148329e+00 4.735748e+00 2.974173e+00 1.955084e+00 1.055983e+00
[16] 4.074498e-01 2.936479e-06

```

These are all positive and non-zero, which confirms that the optimisation routine has found a local maximum of the likelihood.

## 11.2 Check Other Starts for vMF

```

restarts <- pbapply::pblapply(1:100, function(seed){
  start <- rmnlink_cann(p = 3, qs = 3, qe = ncol(xe) + 2, preseed = seed)
  # convert to LinEuc form:
  set.seed(seed+1)
  Qe <- mclust::randomOrthogonalMatrix(ncol(xe)+1, 3-1)
  bigQe <- cbind(0, rbind(0, Qe))
  bigQe[, 1] <- 0
  bigQe[1,1] <- 1
  start$Qe <- bigQe
  start$ce <- 1
  modvMF <- mobius_vMF(y = fulldf %>% select(starts_with("Y")) %>% as.matrix(),
    xs = fulldf %>% select(starts_with("X")) %>% as.matrix(),
    xe = xe %>% as.matrix(),
    fix_qs1 = FALSE, type = "LinEuc",
    start = start)
}, cl = 2)
lapply(restarts, "[", "obj") %>%
  unlist() %>%
  enframe("seed", "objective") %>%
  ggplot()+
  geom_freqpoly(aes(x = objective), bins = 30) +
  geom_vline(xintercept = mod$preest$nlopt$objective, col = "blue") +
  geom_rug(aes(x = objective))

```

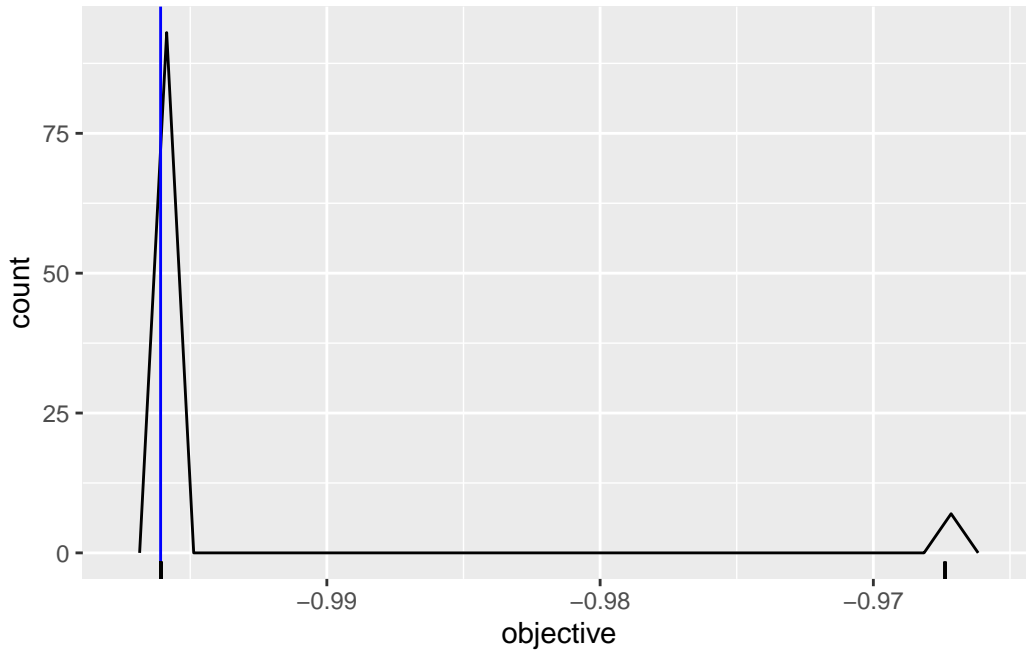

Other initial parameters have not improved on the default initial parameters.

### 11.3 Check Other Starts for SvMF

```
restarts <- pbapply::pblapply(1:100, function(seed){
  # randomly generates a SpEuc-form link
  start <- rmnlink_cann(p = 3, qs = 3, qe = ncol(xestd) + 2, preseed = seed)
  # convert to LinEuc form:
  set.seed(seed+1)
  Qe <- mclust::randomOrthogonalMatrix(ncol(xestd)+1, 5-1)
  bigQe <- cbind(0, rbind(0, Qe))
  bigQe[, 1] <- 0
  bigQe[1,1] <- 1
  start$Qe <- bigQe
  start$ce <- 1
  mobius_SvMF(y = fulldf %>% select(starts_with("Y")) %>% as.matrix(),
              xs = fulldf %>% select(starts_with("X")) %>% as.matrix(),
              xe = xestd %>% as.matrix(),
              type = "LinEuc",
              G01behaviour = "free",
              mean = start)
```

```

}, cl = 2)
badrestarts <- unlist(lapply(restarts, inherits, "try-error"))
restarts <- restarts[!badrestarts]
lapply(restarts, "[", "AIC") %>%
  unlist() %>%
  tibble::enframe("seed", "AIC") %>%
  ggplot()+
  geom_freqpoly(aes(x = AIC), bins = 30) +
  geom_vline(xintercept = mod$AIC, col = "blue") +
  geom_rug(aes(x = AIC))

```

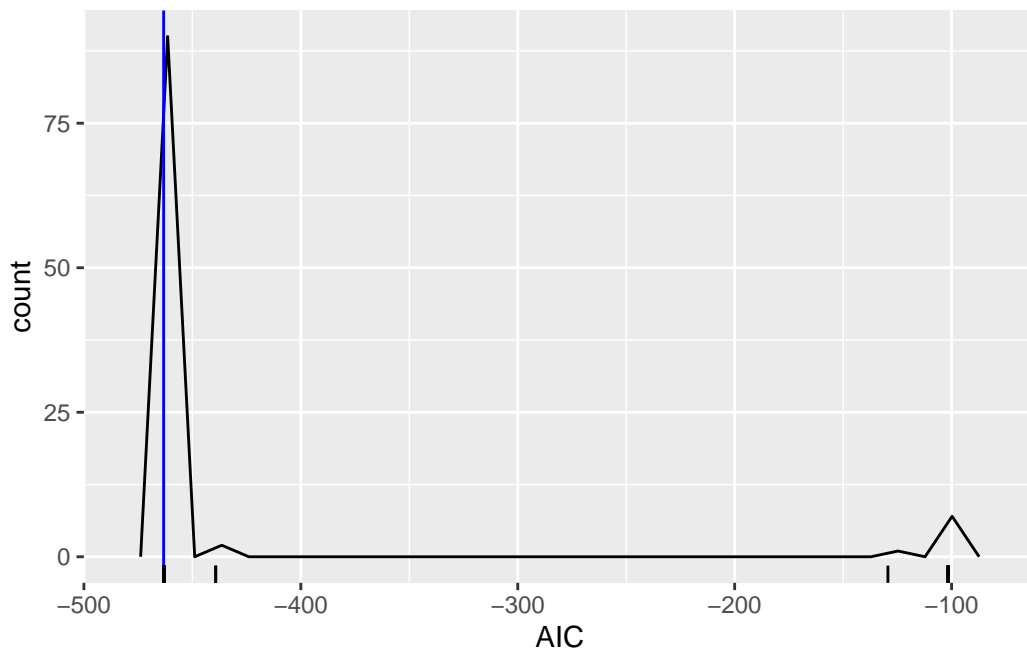

Other initial parameters have not improved on the default initial parameters.
