# Supplementary material for: Regression for spherical responses with linear and spherical covariates using a scaled link function
Source: arXiv:2509.06204 ancillary file (2025-09-07)
Supplement: Supplementary file 2 [file reproduce_earthquakes.pdf]

# Mobius Regression of Earthquake Moment Tensors

Shallow Earthquakes Regions 2 - 4

## Table of contents

|          |                                                                         |           |
|----------|-------------------------------------------------------------------------|-----------|
| <b>1</b> | <b>Preparation</b>                                                      | <b>2</b>  |
| 1.1      | Raw Data . . . . .                                                      | 2         |
| 1.2      | Transform to $S^4$ . . . . .                                            | 3         |
| 1.2.1    | Enforce Trace=0 and Scale=1 . . . . .                                   | 3         |
| 1.2.2    | Moment Tensors as Unit Vectors in $R^5$ . . . . .                       | 5         |
| 1.3      | Hejrani et al (2017)'s Regions . . . . .                                | 6         |
| 1.4      | Keep Only Shallow Earthquakes in Regions 2-4 . . . . .                  | 7         |
| 1.5      | $S^4$ Plot Helpers . . . . .                                            | 7         |
| 1.6      | Pairwise Projections of Earthquake Moment Tensors (SI Figure) . . . . . | 10        |
| 1.7      | Additional Covariates . . . . .                                         | 12        |
| 1.7.1    | Distance to BSSL . . . . .                                              | 12        |
| 1.7.2    | Strike of BSSL . . . . .                                                | 13        |
| 1.8      | Look for Outliers (SI Figure) . . . . .                                 | 15        |
| 1.9      | Remove Outliers . . . . .                                               | 18        |
| 1.10     | Main Figure: Earthquake Locations . . . . .                             | 19        |
| 1.11     | Build covariates . . . . .                                              | 19        |
| <b>2</b> | <b>Default Start for SvMF Regression</b>                                | <b>20</b> |
| <b>3</b> | <b>SI Figure: Random Starts</b>                                         | <b>21</b> |
| <b>4</b> | <b>SI Table: Estimated Parameters</b>                                   | <b>22</b> |
| <b>5</b> | <b>SI Figure: Predictions</b>                                           | <b>25</b> |
| <b>6</b> | <b>Main Figure: Observed and Predicted</b>                              | <b>29</b> |
| <b>7</b> | <b>Angles to <math>b_{01}</math> and <math>\gamma_{01}</math></b>       | <b>30</b> |

|           |                                                      |           |
|-----------|------------------------------------------------------|-----------|
| <b>8</b>  | <b>Predictions in Standardised Coordinates</b>       | <b>31</b> |
| <b>9</b>  | <b>Model Diagnostics</b>                             | <b>36</b> |
| 9.1       | Rotated Residuals (SI Figure) . . . . .              | 36        |
| 9.2       | Residual Mean by Covariates (SI Figure) . . . . .    | 38        |
| 9.3       | Standardised Residuals . . . . .                     | 43        |
| 9.4       | Standardised Residual Distance (SI Figure) . . . . . | 45        |
| 9.5       | Residual Distance (Unstandardised) . . . . .         | 46        |
| <b>10</b> | <b>Likelihood Ratio Test of vMF vs SvMF</b>          | <b>47</b> |
| <b>11</b> | <b>Parametric Bootstrap Regions for a</b>            | <b>51</b> |
| 11.1      | 95% CI for a (SI Table) . . . . .                    | 52        |

# 1 Preparation

## 1.1 Raw Data

This data is copied directly from Hejrani et al (2017) Table 1.

```
raw=read.table(file="./papua20240709.csv",
               header=T,sep="," , numerals = "warn.loss",
               colClasses = c(Origin.Time = "character"))
head(raw) %>%
  mutate(Origin.Time = paste0(substr(`Origin.Time`, 1, 6),"..")) %>%
  rename(Lon = Longitude,
         Lat = Latitude) %>%
  knitr::kable() %>%
  kableExtra::kable_styling(font_size = 8)
```

| Number | Origin.Time | Lon   | Lat  | Depth | Mrr   | Mtt   | Mff   | Mrt   | Mrf   | Mtf   | Exp | Mw  | Dcper |
|--------|-------------|-------|------|-------|-------|-------|-------|-------|-------|-------|-----|-----|-------|
| 1      | 200602..    | 149.8 | -6.4 | 35    | 2.86  | -2.83 | -0.03 | 1.14  | 0.17  | 0.02  | 17  | 5.6 | 97.4  |
| 2      | 200603..    | 150.0 | -4.8 | 11    | -2.93 | 3.81  | -0.88 | -1.79 | -2.49 | 1.05  | 17  | 5.7 | 96.8  |
| 3      | 200603..    | 151.4 | -6.0 | 27    | 1.76  | -0.22 | -1.54 | -0.52 | 0.24  | 0.77  | 17  | 5.4 | 94.4  |
| 4      | 200603..    | 143.2 | -3.2 | 3     | 7.65  | -5.29 | -2.36 | 6.74  | 5.21  | 8.99  | 17  | 6.0 | 75.4  |
| 5      | 200605..    | 154.8 | -7.8 | 7     | -0.15 | 1.29  | -1.14 | 0.69  | -0.57 | 0.36  | 17  | 5.4 | 95.8  |
| 6      | 200606..    | 151.8 | -5.2 | 43    | 9.63  | -8.84 | -0.78 | 3.01  | 0.92  | -2.24 | 16  | 5.3 | 96.0  |

In this raw data:

- **Origin.Time**. Hejrani references the GCMT project for origin times. Though not explicitly in Hejrani et al (2017), it seems this column is the format that GCMT uses for modern earthquakes, which is `XYYYMMDDhhmmZ` where `X` is the type of data used, `Z` is for distinguishing events at the same time (day?) and the stuff in between is time.
- **Number** relates uniquely to increasing origin time.
- **Lon** and **Lat** are the Longitude and Latitude of the earthquake
- **Depth** is the depth (in kilometres) of the earthquake
- **M\*\*** are scaled elements of the earthquake moment tensors where **r**, **t**, **f** represent basis directions.
- **Mw \* 10<sup>Exp</sup>** is a magnitude.
- **Dcper** is related to how close the earthquake is to a pure double-couple.

For later let's record the names of the **M\*\*** columns in the same order as the symmetric-matrix vectorisation function `vech`:

```
elementnames <- c("Mrr", "Mrt", "Mrf",
                  "Mtt", "Mtf",
                  "Mff")
```

## 1.2 Transform to $S^4$

### 1.2.1 Enforce Trace=0 and Scale=1

The moment tensors have traces that are nearly 0.

```
traces <- rowSums(raw[, c("Mrr", "Mtt", "Mff")])
traces %>%
  tibble::enframe(value = "trace") %>%
  ggplot() +
  geom_histogram(aes(x = trace), bins = 30) +
  geom_rug(aes(x = trace))
```

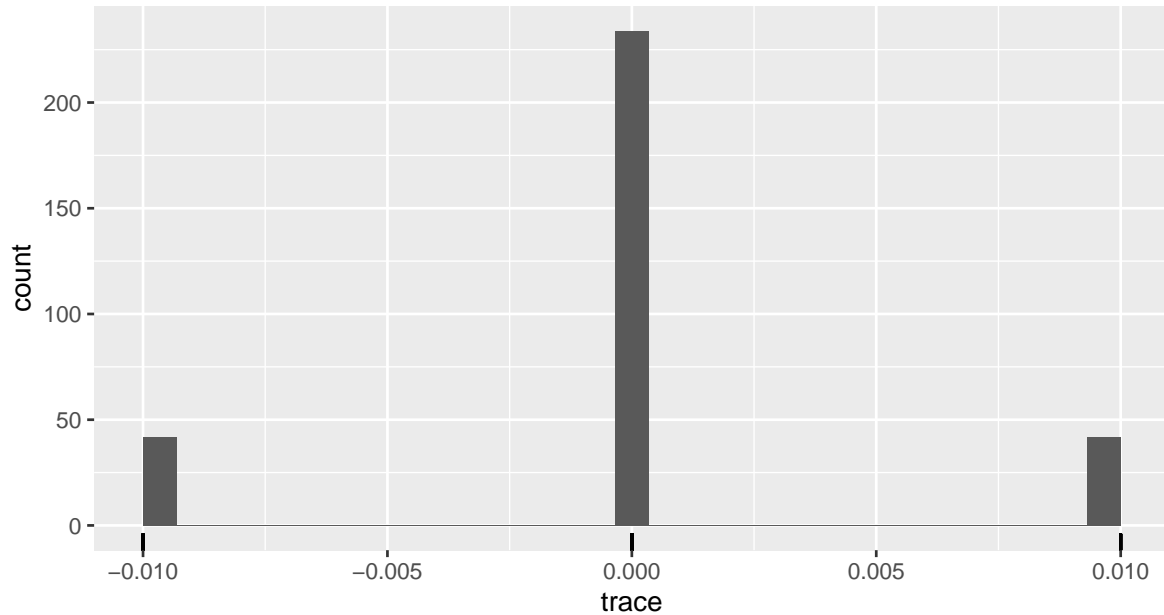

Here I'll make the trace exactly zero.

```
stddf <- raw %>%
  mutate(Mff = -Mrr - Mtt)
```

Now we scale the moment tensors to have a Frobenius norm of 1. The function `gettr2()` below is a fast way to compute the square of the Frobenius norm without winding the 6 `M**` columns up into individual 3 x 3 matrices.

```
gettr2 <- function(ms){
  I2 <- ms[, 1] * ms[, 4] + ms[, 4] * ms[, 6] + ms[, 1] * ms[, 6] -
    ms[, 2]^2 - ms[, 5]^2 - ms[, 3]^2
  I1 <- ms[, 1] + ms[, 4] + ms[, 6] #trace
  tr2 <- I1^2 - 2*I2
  return(tr2)
}
Fnorm <- sqrt(gettr2(stddf[, elementnames]))
stddf <- stddf %>%
  mutate(Fnorm = Fnorm) %>%
  mutate(across(starts_with("M"), ~.x/Fnorm))
```

Lets verify the result of these transformations on the first earthquake.

```

elementvalues <- unlist(stddf[1, elementnames])
tmpM <- matrix(NA, 3, 3)
tmpM[lower.tri(tmpM, diag = TRUE)] <- elementvalues
tmpM[upper.tri(tmpM)] <- t(tmpM)[upper.tri(tmpM)]
colnames(tmpM) <- rownames(tmpM) <- c("r", "t", "f")

```

```
elementvalues
```

|  | Mrr         | Mrt         | Mrf         | Mtt          | Mtf         | Mff          |
|--|-------------|-------------|-------------|--------------|-------------|--------------|
|  | 0.658783349 | 0.262591964 | 0.039158451 | -0.651873034 | 0.004606877 | -0.006910315 |

```
tmpM
```

|   | r          | t            | f            |
|---|------------|--------------|--------------|
| r | 0.65878335 | 0.262591964  | 0.039158451  |
| t | 0.26259196 | -0.651873034 | 0.004606877  |
| f | 0.03915845 | 0.004606877  | -0.006910315 |

```
sqrt(sum(tmpM^2))
```

```
[1] 1
```

```
sum(diag(tmpM))
```

```
[1] -3.035766e-17
```

The trace and norm are exactly 0 and 1 as desired.

### 1.2.2 Moment Tensors as Unit Vectors in $R^5$

The diagonal elements must sum to zero, which puts them on a plane through the origin. I'll use the Helmert submatrix to express these diagonal elements with respect to an orthonormal basis on this plane. The plane is two dimensions, so I'll call these new coordinates **s1** and **s2**.

```

H <- rbind(c(1,-1, 0), c(1,1,-2))
H <- H/sqrt(rowSums(H^2))
diagproj <- t(H %*% t(stddf[, c("Mrr", "Mtt", "Mff"))])
colnames(diagproj) <- c("s1", "s2")

```

I'll scale the off diagonal elements by  $\sqrt{2}$  because off-diagonal elements are counted twice in the Frobenius norm.

```
offdiag <- stddf %>%
  mutate(sMrt = sqrt(2) * Mrt,
         sMrf = sqrt(2) * Mrf,
         sMtf = sqrt(2) * Mtf) %>%
  select(sMrt, sMrf, sMtf)
```

Combined these are unit vectors in  $R^5$

```
sqrt(rowSums(cbind(diagproj, offdiag)^2))
```

[illegible]

Lets add these unit vectors into full data frame

```
s4df <- bind_cols(diagproj, offdiag, raw)
```

### 1.3 Hejrani et al (2017)'s Regions

Here I have captured the regions from Fig 16 of Hejrani et al (2017) by visual assessment.

```
ptmatrix <- function(xmin, xmax, ymin, ymax){
  matrix(c(xmin, ymax,
           xmax, ymax,
           xmax, ymin,
           xmin, ymin,
           xmin, ymax), byrow = TRUE, ncol = 2)
}

regions <- st_sfc(st_polygon(list(ptmatrix(141, 144, -4, -2))),
```

```

      st_polygon(list(ptmatrix(144, 147.3, -4, -2))),
      st_polygon(list(ptmatrix(147.3, 150.3, -4, -2.5))),
      st_polygon(list(ptmatrix(150.3, 152.5, -4.1, -3))),
      st_polygon(list(ptmatrix(146.1, 151.5, -7.1, -5.7))),
      st_polygon(list(ptmatrix(151.5, 153.5, -6.8, -4.7))),
      st_polygon(list(ptmatrix(153.5, 156.7, -8.5, -5))),
      st_polygon(list(ptmatrix(156.7, 159, -10, -8))),
    crs = 4326)
regions <- st_sf(region = factor(1:8, ordered = TRUE), geom = regions)

```

## 1.4 Keep Only Shallow Earthquakes in Regions 2-4

The below keeps only earthquakes in regions 2 to 4 with depth smaller than 20. It assumes that the longitude and latitude are follow the GPS coordinate system.

```

s4df <- sf::st_as_sf(s4df, coords = c("Longitude", "Latitude"), remove = FALSE)
sf::st_crs(s4df) <- 4326
s4df <- st_intersection(s4df, regions)

```

Warning: attribute variables are assumed to be spatially constant throughout all geometries

```

s4df <- mutate(s4df, region = as.factor(region))
s4df <- s4df %>%
  filter(region %in% 2:4) %>%
  filter(Depth <= 20)
nrow(s4df)

```

```
[1] 50
```

## 1.5 $S^4$ Plot Helpers

Below makes circles for plotting the edge of  $S^4$  later.

```

# Create data for the unit circle
theta <- seq(0, 2 * pi, length.out = 100)
circle_df <- data.frame(x = cos(theta), y = sin(theta))
colpairs <- #combn(paste0("Y", 1:5), 2, simplify = FALSE)
expand.grid(paste0("Y", 1:5), paste0("Y", 1:5)) %>%

```

```

filter(Var1 != Var2) %>%
mutate(Var1 = as.character(Var1), Var2 = as.character(Var2)) %>%
rowwise() %>%
mutate(pair = list(c(Var1, Var2))) %>%
select(pair) %>%
unlist(recursive = FALSE)
pair_dfs <- lapply(colpairs, function(pair) {
  Aname <- pair[1]
  Bname <- pair[2]
  circle_df %>%
    rename(A = x, B = y) %>%
    mutate(pair1=Aname,
           pair2=Bname,
           pair = paste(pair, collapse = "-"))
})
circle_df_long <- bind_rows(pair_dfs)

```

And the following is useful for orthogonal projection of locations on to pairs of axes:

```

pivot_coordpairs <- function(df,
                             coordnames = paste0("Y",1:5),
                             colpairs = combn(coordnames, 2, simplify = FALSE)){
  pair_dfs <- lapply(colpairs, function(pair) {
    Aname <- pair[1]
    Bname <- pair[2]
    df %>%
      # copy pair values
      mutate(A = .data[[Aname]],
             B = .data[[Bname]]) %>%
      mutate(pair1=Aname,
             pair2=Bname,
             pair = paste(pair, collapse = "-"))
  })
  pairsdf <- bind_rows(pair_dfs)
  attr(pairsdf, "coordnames") <- coordnames
  pairsdf
}

pairedplotggprep <- function(df){
  # rename circle_df_long to coordnames
  dict <- attr(df, "coordnames")
  names(dict) <- paste0("Y", 1:length(dict))
  circle_df_long <- circle_df_long %>%

```



```

mutate(
  pair1 = dict[pair1],
  pair2 = dict[pair2],
  pair = paste0(pair1,"-",pair2))

# nicer strip labels
label_map <- c(
  s1 = "(Mrr - Mtt)/sqrt(2)",
  s2 = "(Mrr + Mtt - 2*Mff)/sqrt(6)",
  sMrf = "Mrf / sqrt(2)",
  sMrt = "Mrt / sqrt(2)",
  sMtf = "Mtf / sqrt(2)",
  Y1 = "Y1",
  Y2 = "Y2",
  Y3 = "Y3",
  Y4 = "Y4",
  Y5 = "Y5",
  r1 = "r1",
  r2 = "r2",
  r3 = "r3",
  r4 = "r4"
)

#now do plotting prep
ggplot(data = df, mapping = aes(x=A, y=B)) +
facet_grid(vars(pair2),
  vars(pair1),
  switch = "both",
  labeller = as_labeller(label_map, label_parsed)) +
geom_path(data = ~(circle_df_long %>% filter(pair %in% .x$pair)),
  mapping = aes(x=A,y=B),
  inherit.aes = FALSE,
  color = "grey") +
coord_fixed(xlim = c(-1.01,1.01), ylim = c(-1.01,1.01), expand = FALSE) +
theme_minimal() +
theme(strip.text.y = element_text(angle = 90),
  strip.placement = "outside",
  axis.title = element_blank(),
  axis.text = element_blank(),
  axis.line = element_line(arrow = grid::arrow(type = "closed",
    angle = 10,
    length = unit(10, "points"))),

```

```

                                linewidth = 0.2),
  panel.grid = element_blank(),
  legend.position = "bottom")
}

```

## 1.6 Pairwise Projections of Earthquake Moment Tensors (SI Figure)

```

s4df %>%
  pivot_coordpairs(coordnames = c("s1", "s2", "sMrf", "sMrt", "sMtf")) %>%
  pairedplotggprep() +
  geom_point(aes(col = Longitude)) +
  scale_shape_manual(guide = "none", values = c(4, 16)) +
  scale_color_viridis_c()

```

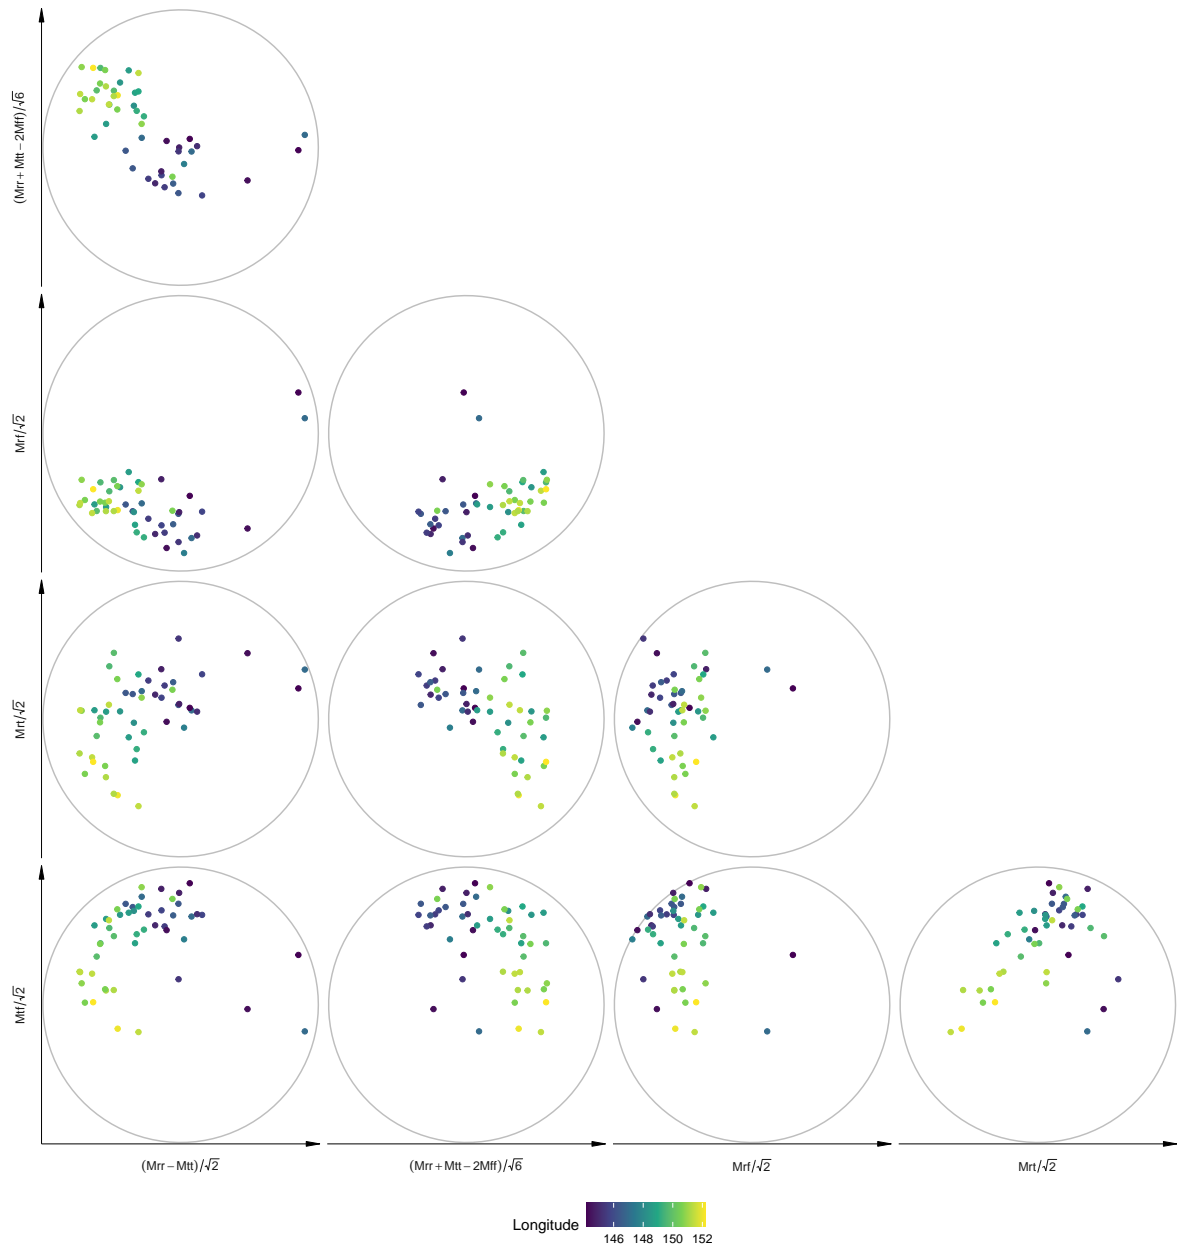

```
ggsave("earthq_mtensors.pdf", width = 12, height = 13)
```

## 1.7 Additional Covariates

For each earthquake we find the distance to the BSSL and also the direction (up to  $\pm\pi$ ) of the fault at this closest point. This direction is known as the strike in seismology (For BSSL, the fault plane is vertical so strike may as well be below  $\pi$ ).

### 1.7.1 Distance to BSSL

Plate information was obtained from github <https://github.com/fraxen/tectonicplates>.

```
tmp <- paste0("https://github.com/fraxen/tectonicplates/raw/refs/heads/master/PB2002_boundar")
  lapply(function(x){download.file(x, basename(x))})
```

```
world <- ne_countries(scale = "medium", returnclass = "sf")
tecbound <- st_read("PB2002_boundaries.shp")
```

```
Reading layer `PB2002_boundaries' from data source
  `/home/kassel/Documents/professional/ANU_Compositional/SphericalRegression_mobius/SphRegByL
  using driver `ESRI Shapefile'
Simple feature collection with 241 features and 6 fields
Geometry type: LINESTRING
Dimension:      XY
Bounding box:   xmin: -180 ymin: -66.1632 xmax: 180 ymax: 86.8049
Geodetic CRS:   WGS 84
```

```
mat <- st_intersects(tecbound, st_as_sfc(st_bbox(s4df)))
tecbound <- tecbound[apply(mat, 1, any), ]
tecbound <- tecbound %>%
  mutate(NiceName = case_match(
    Name,
    "NB-SB" ~ "BSSL",
    "NB-MN" ~ "BSSL",
    "MN-SB" ~ "BSSL",
    "NB-SB" ~ "BSSL",
    .default = "Other"
  ))
```

```
dist_BSSL <- tecbound %>%
  filter(NiceName == "BSSL") %>%
  st_union() %>%
```

```

  st_distance(s4df) %>%
  drop() %>%
  units::drop_units()
s4df <- s4df %>%
  mutate(dist = dist_BSSL)

```

### 1.7.2 Strike of BSSL

The strike (up to  $\pm\pi$ ) of the faults at the closest point to each earthquake.

First need to split the faults into segments

```

tecbound_interest <- tecbound %>%
  filter(NiceName == "BSSL")
teccoords <- tecbound_interest %>%
  st_coordinates()
strike <- teccoords %>%
  as_tibble() %>%
  tibble::rowid_to_column() %>%
  st_as_sf(coords = c("X", "Y"), crs = st_crs(tecbound)) %>%
  lwgeom::st_geod_azimuth() %>%
  units::drop_units()
# make strike between 0 and 2pi
strike[which(strike < 0)] <- strike[which(strike < 0)] + 2*pi
# get segments as sf objects
segs <- cbind(teccoords[-nrow(teccoords), c("X", "Y")], teccoords[-1, c("X", "Y")]) %>%
  apply(1, function(vec){
    st_linestring(matrix(vec, 2, 2, byrow = TRUE))
  }, simplify = FALSE) %>%
  st_as_sfc(crs = st_crs(tecbound))
segs <- st_sf(strike = strike, fault = teccoords[-nrow(teccoords), "L1"], geometry = segs)
# remove the bearings corresponding to jumping between faults
segs <- segs[teccoords[-nrow(teccoords), "L1"] - teccoords[-1, "L1"] >= -0.5, ]

# L1 refers to the feature so can get back to plate names etc
segs$FaultName <- tecbound_interest$Name[segs$fault]
segs$NiceName <- tecbound_interest$NiceName[segs$fault]

segs <- segs %>%
  mutate(strike = case_when(strike > pi ~ strike - pi,
                             TRUE ~ strike))

```

```
segs %>%
  # mutate(strike = cut(strike, c(0,1.7,2.5, pi), include.lowest = TRUE)) %>%
  ggplot() +
  geom_sf(aes(col = strike), linewidth = 2) +
  scale_color_viridis_c() +
  coord_sf(xlim = c(144.0, 153), ylim = c(-4.5, -2))
```

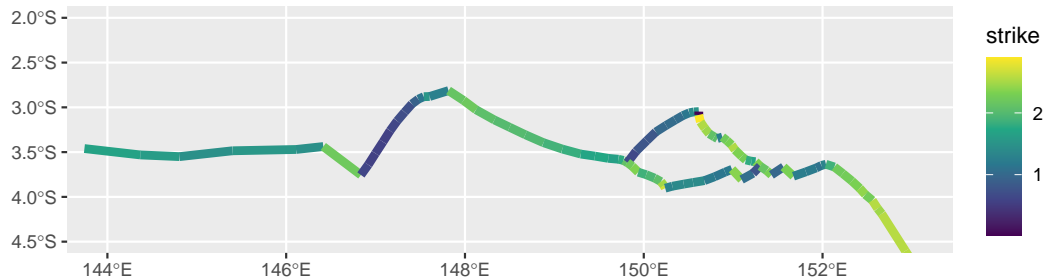

Find closest segment to each earthquake and use that for strike.

```
segidx <- st_nearest_feature(s4df, segs)
strike_BSSL <- segs$strike[segidx, drop = TRUE]
s4df <- bind_cols(s4df, fstrike = strike_BSSL)
```

Below plots the assigned fault's strike (`fstrike`) closest to each earthquake

```
segs %>%
  ggplot() +
  geom_sf(aes(col = strike), linewidth = 2) +
  geom_point(data = s4df,
    aes(x = Longitude, y = Latitude, fill = fstrike),
    shape = 21,
    show.legend = FALSE) +
  scale_color_viridis_c(name = "Strike", limits = range(segs$strike)) +
  scale_fill_viridis_c(name = "Strike", limits = range(segs$strike)) +
  coord_sf(xlim = c(144.0, 153), ylim = c(-4.5, -2))
```

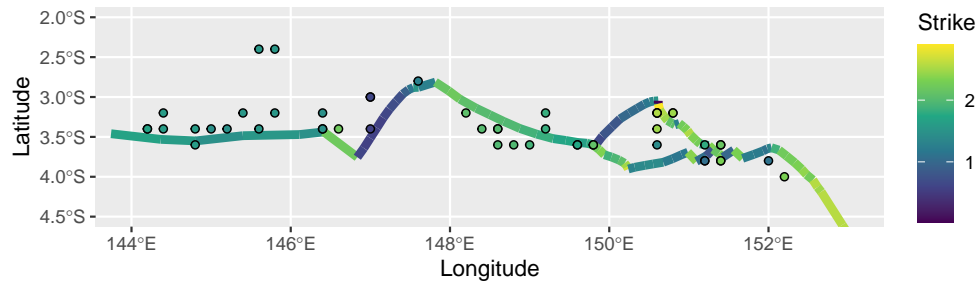

## 1.8 Look for Outliers (SI Figure)

Here I'll look for outliers. I'll view the moment tensors orthogonally projected onto axes determined by the first and second moment of the data such that the mean moment tensor has  $Y1=1$  and the covariance of the data in  $Y2...Y5$  coordinates is diagonal. The moment tensors according to these axes are obtained using `standardise_sph()`.

Point colour is given by earthquake longitude. Background colour is the average earthquake longitude for that part of projected  $S^4$ . The identified outliers are labelled.

```
outliers <- c(
  "182" = "general",
  "306" = "general",
  "76" = "general",
  "254" = "general",
  "169" = "general",
  "87" = "general",
  "175" = "longitude",
  "260" = "longitude"
)
outliers <- outliers %>%
  tibble::enframe(name = "Number", value = "outlier") %>%
  mutate(Number = as.integer(Number))

s4df %>%
  st_drop_geometry() %>%
  mutate(stdcoords = as_tibble(
    standardise_sph(as.matrix(across(c(s1, s2, sMrt, sMrf, sMtf)))),
    .name_repair = "minimal")) %>%
  tidyr::unnest_wider(stdcoords, names_sep = "") %>%
  rename_with(~gsub("stdcoords", "Y", .)) %>%
  left_join(outliers, by = "Number") %>%
  pivot_coordpairs(coordnames = paste0("Y", 1:5)) %>%
```

```

pairedplotggprep() +
stat_summary_2d(fun = mean,
                aes(z = Longitude, fill = after_stat(value)),
                bins = 10) +
scale_fill_viridis_c(name = "Longitude") +
geom_point(aes(fill = Longitude), size = 2, shape = 21) +
ggrepel::geom_label_repel(aes(label = Number,
                              col = as.factor(outlier)),
                          data = ~filter(.x, !is.na(outlier)),
                          label.padding = 0.1,
                          min.segment.length = 0,
                          box.padding = 1,
                          show.legend = FALSE) +
scale_colour_manual(values = c("black", "grey"))

```



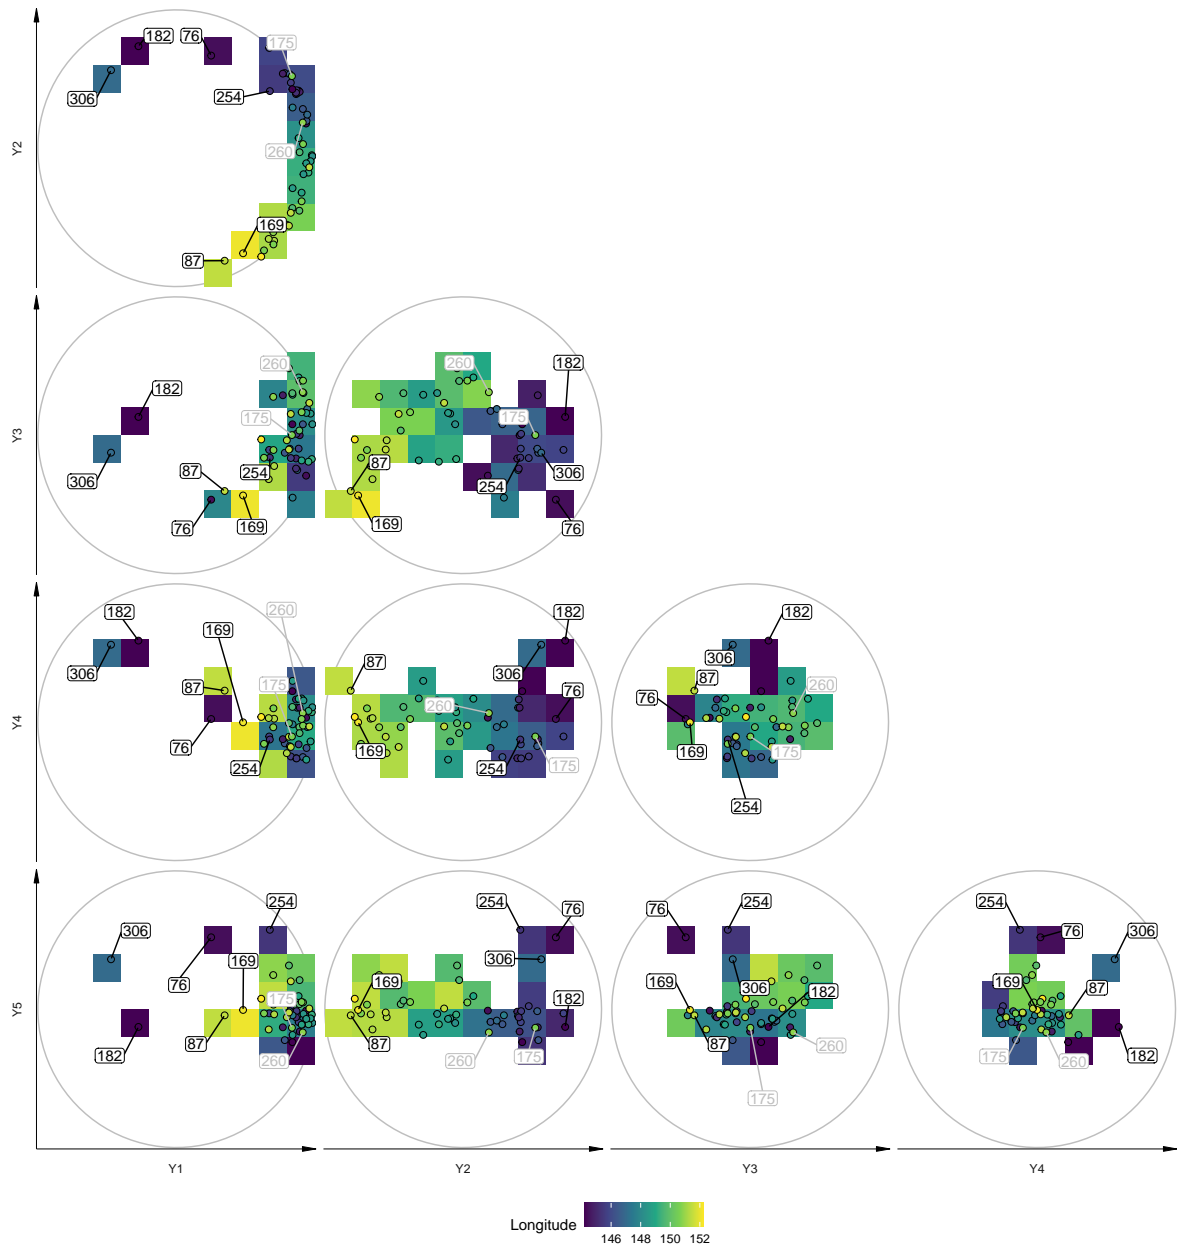

```
ggsave("earthq_mtensors_outlier.pdf", width = 12, height = 13)
```

From these plots we can see 6 earthquakes very different to the rest in at least some of the coordinates Y1 - Y5. Earthquakes 182, 306, 76, 87 and 169 were outlying in Y1. Earthquake 254 is an outlier in Y5. Furthermore, earthquake 175 and to a lesser extent, earthquake 260, have high longitude, but have moment tensors close to low longitude earthquakes.

There also appears to be a shift in earthquake moment tensors with longitude < 148 (blue) vs other earthquakes (green-yellow), which we will incorporate into regression later.

## 1.9 Remove Outliers

The outliers by region are:

```
outliers <- outliers %>% #remove duplicates
  group_by(Number) %>%
  summarise(outlier = paste0(outlier, collapse = ","))

s4df %>%
  left_join(outliers, by = "Number") %>%
  filter(!is.na(outlier)) %>%
  st_drop_geometry() %>%
  select(Number, region, outlier) %>%
  arrange(region)
```

|   | Number | region | outlier   |
|---|--------|--------|-----------|
| 1 | 76     | 2      | general   |
| 2 | 182    | 2      | general   |
| 3 | 254    | 2      | general   |
| 4 | 306    | 2      | general   |
| 5 | 87     | 4      | general   |
| 6 | 169    | 4      | general   |
| 7 | 175    | 4      | longitude |
| 8 | 260    | 4      | longitude |

```
s4df_clean <- s4df %>%
  left_join(outliers, by = "Number") %>%
  filter(is.na(outlier))
nrow(s4df_clean)
```

```
[1] 42
```

```
s4df_clean$Depth %>% as.factor() %>% summary()
```

```
3  7 11 15 19
5 14 11  9  3
```

## 1.10 Main Figure: Earthquake Locations

```
ggplot() +  
  geom_sf(data = world) +  
  geom_point(data = s4df %>% left_join(outliers, by = "Number") %>% filter(!is.na(outlier)),  
            aes(x = Longitude, y = Latitude),  
            shape = 4,  
            position = position_jitter(width = 0.05, height = 0.05, seed = 1),  
            show.legend = FALSE) +  
  geom_point(data = s4df %>% left_join(outliers, by = "Number") %>% filter(is.na(outlier)),  
            aes(x = Longitude, y = Latitude, col = Longitude),  
            position = position_jitter(width = 0.05, height = 0.05, seed = 1),  
            show.legend = FALSE) +  
  scale_color_viridis_c() +  
  # scale_shape_manual(values = c(4, 16)) +  
  geom_sf(data = tecbound %>% filter(NiceName != "Other"), aes(lty = NiceName), show.legend =  
  # geom_sf(data = regions %>% filter(region %in% 2:4), fill = NA, show.legend = FALSE) +  
  scale_linetype_manual(values = c(NGT = "dashed", BSSL = "solid", Other = "dotted")) +  
  theme_bw() +  
  theme(axis.title = element_blank()) +  
  coord_sf(xlim = c(144.0, 153), ylim = c(-4.5, -2))
```

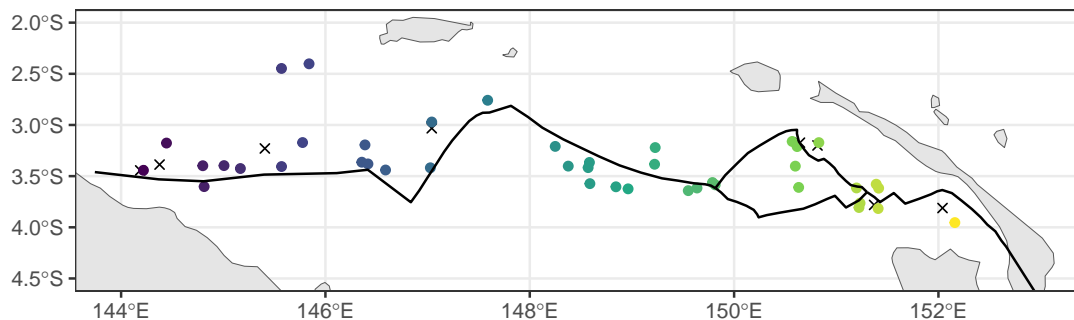

```
ggsave("earthquakelocations.pdf", width = 7, height = 2)
```

Caption: Shallow earthquake locations near the Bismarck Sea Seismic Lineation (solid line). Some jitter has been introduced because 12 are colocated.

## 1.11 Build covariates

Scale and center all Euclidean covariates to have mean 0 and sd of 1.

```

xe <- s4df_clean %>%
  st_drop_geometry() %>%
  select(fstrike,
         Latitude,
         Longitude
        ) %>%
  mutate(Longitude.L148 = (Longitude > 148) * Longitude) %>%
  as.matrix()
xestd <- xe %>%
  scale() |>
  as_tibble()
cor(xestd)

```

|                | fstrike    | Latitude   | Longitude  | Longitude.L148 |
|----------------|------------|------------|------------|----------------|
| fstrike        | 1.0000000  | -0.1801471 | 0.4575706  | 0.5725929      |
| Latitude       | -0.1801471 | 1.0000000  | -0.4904033 | -0.5022031     |
| Longitude      | 0.4575706  | -0.4904033 | 1.0000000  | 0.8926280      |
| Longitude.L148 | 0.5725929  | -0.5022031 | 0.8926280  | 1.0000000      |

## 2 Default Start for SvMF Regression

```

mod_SvMF <- mobius_SvMF(s4df_clean %>%
  select(s1, s2, sMrt, sMrf, sMtf) %>%
  st_drop_geometry() %>%
  as.matrix(),
  xs = NULL,
  xe = xestd %>% as.matrix(),
  type = "LinEuc",
  G01behaviour = "free")

```

Warning in tape\_ld\_Mobius\_SvMF\_partran\_notal(omvec = om0vec, k = preplist\$k, :  
This function approximates the vMF normalising constant when p!=3.

```
mod_SvMF$k
```

```
[1] 56.94665
```

```
mod_SvMF$AIC
```

```
[1] -137.0572
```

```
mod_SvMF$a
```

```
1.0000000 2.0910088 1.2106586 0.9542765 0.4139503
```

```
mod_SvMF$DoF
```

```
[1] 38
```

### 3 SI Figure: Random Starts

```
restarts <- pbapply::pblapply(1:100, function(seed){
  # randomly generates a SpEuc-form link
  start <- rmnlink_cann(p = 5, qs = 0, qe = ncol(xestd) + 2, preseed = seed)
  # convert to LinEuc form:
  set.seed(seed+1)
  Qe <- mclust::randomOrthogonalMatrix(ncol(xestd)+1, 5-1)
  bigQe <- cbind(0, rbind(0, Qe))
  bigQe[, 1] <- 0
  bigQe[1,1] <- 1
  start$Qe <- bigQe
  start$ce <- 1
  mobius_SvMF(s4df_clean %>%
    select(s1, s2, sMrt, sMrf, sMtf) %>%
    st_drop_geometry() %>%
    as.matrix(),
    xs = NULL,
    xe = xestd %>% as.matrix(),
    type = "LinEuc",
    G01behaviour = "free",
    mean = start)
}, cl = 2)
badrestarts <- unlist(lapply(restarts, inherits, "try-error"))
restarts <- restarts[!badrestarts]
```

```
lapply(restarts, "[", "AIC") %>%
  unlist() %>%
  tibble::enframe("seed", "AIC") %>%
  ggplot()+
  geom_histogram(aes(x = AIC), bins = 30) +
  geom_vline(xintercept = mod_SvMF$AIC, col = "blue") +
  geom_rug(aes(x = AIC))
```

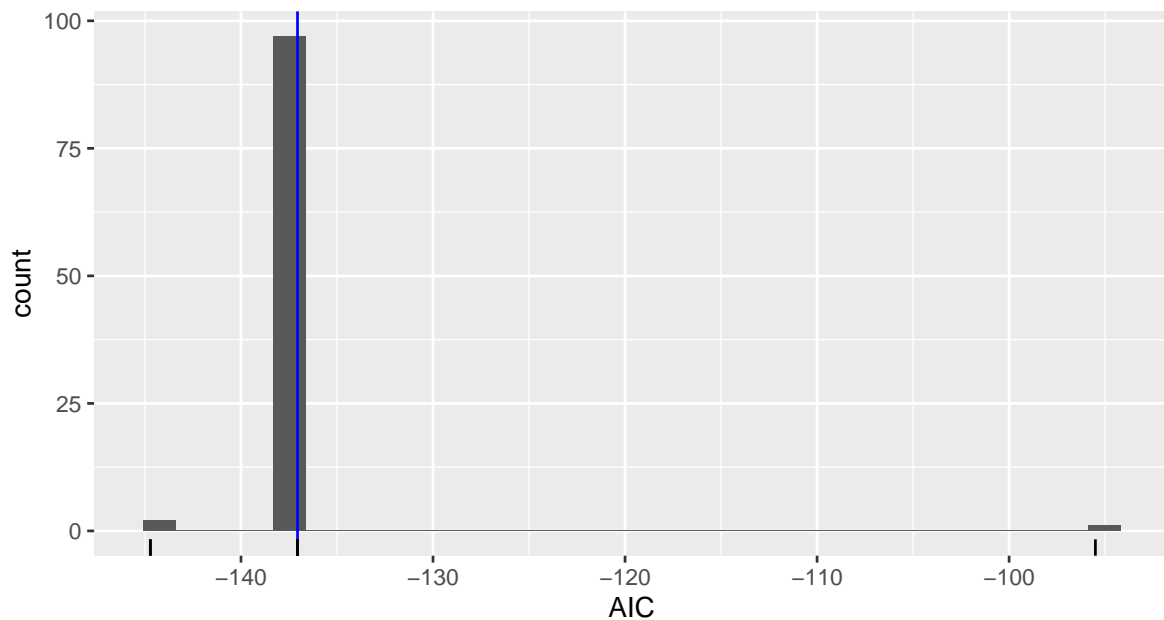

```
ggsave("earthq_restarts.pdf", width = 7, height = 5)
```

```
idx <- which.min(lapply(restarts, "[", "AIC") %>% unlist())
mod_SvMF <- restarts[[idx]]
```

## 4 SI Table: Estimated Parameters

Below is the estimated concentration, the AIC and degrees of freedom of this regression.

```
mod_SvMF$k
```

```
[1] 59.31133
```

```
mod_SvMF$AIC
```

```
[1] -144.7217
```

```
mod_SvMF$DoF
```

```
[1] 38
```

```
df <- data.frame(t(mod_SvMF$a))
colnames(df) <- 1:ncol(df)
mykbl <- df %>%
  mutate(across(everything(), ~formatC(.x, digits = 2, format = "f"))) %>%
  kbl(booktabs = TRUE, position = "!h", escape = FALSE, format = "latex") %>%
  add_header_above(c("Scales" = ncol(df)), escape = FALSE)
mykbl
```

| Scales |      |      |      |      |
|--------|------|------|------|------|
| 1      | 2    | 3    | 4    | 5    |
| 1.00   | 2.08 | 1.40 | 1.00 | 0.34 |

```
df <- data.frame(mod_SvMF$G0)
label_map <- c(
  s1 = "(Mrr - Mtt)/$\sqrt{2}$",
  s2 = "(Mrr + Mtt - 2Mff)/$\sqrt{6}$",
  sMrf = "Mrf /$\sqrt{2}$",
  sMrt = "Mrt /$\sqrt{2}$",
  sMtf = "Mtf /$\sqrt{2}$"
)
row.names(df) <- label_map[row.names(df)]
colnames(df) <- c("$\gamma_{01}$", "$\gamma_{02}$", "$\gamma_{03}$", "$\gamma_{04}$", "$\gamma_{05}$")
mykbl <- df %>%
  mutate(across(everything(), ~formatC(.x, digits = 2, format = "f"))) %>%
  kbl(booktabs = TRUE, position = "!h", escape = FALSE, format = "latex")
mykbl
```

|                               | $\gamma_{01}$ | $\gamma_{02}$ | $\gamma_{03}$ | $\gamma_{04}$ | $\gamma_{05}$ |
|-------------------------------|---------------|---------------|---------------|---------------|---------------|
| $(Mrr - Mtt)/\sqrt{2}$        | 0.13          | -0.51         | 0.21          | 0.81          | -0.13         |
| $(Mrr + Mtt - 2Mff)/\sqrt{6}$ | 0.22          | 0.51          | -0.59         | 0.49          | 0.31          |
| $Mrt/\sqrt{2}$                | -0.10         | 0.49          | 0.75          | 0.19          | 0.38          |
| $Mrf/\sqrt{2}$                | 0.78          | 0.28          | 0.20          | -0.08         | -0.51         |
| $Mtf/\sqrt{2}$                | -0.56         | 0.39          | -0.04         | 0.24          | -0.69         |

```
cann <- as_mnlink_cann(mod_SvMF$mean)
```

```
df <- data.frame(cann$Be)
colnames(df) <- paste0("col", 1:ncol(df))
mykbl <- df %>%
  mutate(across(everything(), ~round(.x, 2))) %>%
  mutate(across(everything(), as.character)) %>%
  kbl(booktabs = TRUE, position = "!h", escape = FALSE, format = "latex",
      row.names = NA,
      col.names = NULL) %>%
  add_header_above(c("$B_e$" = ncol(df)), escape = FALSE)
mykbl
```

| $B_e$ |      |      |      |
|-------|------|------|------|
| 2.76  | 0    | 0    | 0    |
| 0     | 1.39 | 0    | 0    |
| 0     | 0    | 0.59 | 0    |
| 0     | 0    | 0    | 0.06 |

Below I ignore a dummy zero-valued covariate that is automatically added by the software for compatibility with a link that has a denominator below  $B_e R_e^\top$  (“SpEuc” type link).

```
df <- data.frame(cann$Qe[-1, -1])
colnames(df) <- paste0("col", 1:ncol(df))
rownames(df)[1] <- "Strike"
mykbl <- df %>%
  mutate(across(everything(), ~round(.x, 2))) %>%
  mutate(across(everything(), as.character)) %>%
  kbl(booktabs = TRUE, position = "!h", escape = FALSE, format = "latex",
      row.names = TRUE,
      col.names = NULL) %>%
  add_header_above(c(" " = 1, "$R_e$" = ncol(df)), escape = FALSE)
mykbl
```



|                | $R_e$ |       |       |       |
|----------------|-------|-------|-------|-------|
| Strike         | 0.07  | 0.05  | 0.21  | -0.97 |
| Latitude       | 0.02  | 0.04  | -0.14 | 0.09  |
| Longitude      | 0.49  | 0.08  | -0.84 | -0.16 |
| Longitude.L148 | -0.57 | 0.78  | -0.24 | -0.06 |
| ones           | -0.65 | -0.62 | -0.41 | -0.17 |

```
label_map <- c(
  s1 = "(Mrr - Mtt)/$\sqrt{2}$",
  s2 = "(Mrr + Mtt - 2Mff)/$\sqrt{6}$",
  sMrf = "Mrf /$\sqrt{2}$",
  sMrt = "Mrt /$\sqrt{2}$",
  sMtf = "Mtf /$\sqrt{2}$"
)
df <- data.frame(cann$P)
row.names(df) <- label_map[row.names(df)]
mykbl <- df %>%
  mutate(across(everything(), ~round(.x, 2))) %>%
  mutate(across(everything(), as.character)) %>%
  kbl(booktabs = TRUE, position = "!h", escape = FALSE, format = "latex",
      col.names = NULL) %>%
  add_header_above(c(" " = 1, "$B_0$" = ncol(df)), escape = FALSE)
mykbl
```

|                               | $B_0$ |       |       |      |       |
|-------------------------------|-------|-------|-------|------|-------|
| $(Mrr - Mtt)/\sqrt{2}$        | 0.05  | 0.55  | -0.13 | 0.41 | 0.72  |
| $(Mrr + Mtt - 2Mff)/\sqrt{6}$ | -0.04 | -0.5  | 0.7   | 0.02 | 0.5   |
| $Mrt/\sqrt{2}$                | 0.24  | -0.46 | -0.22 | 0.81 | -0.17 |
| $Mrf/\sqrt{2}$                | 0.27  | 0.48  | 0.65  | 0.29 | -0.43 |
| $Mtf/\sqrt{2}$                | -0.93 | 0.07  | 0.09  | 0.31 | -0.15 |

## 5 SI Figure: Predictions

```
get_predobspairsdf_nat <- function(mod,
  extra = NULL,
  colpairs = combn(c("s1", "s2", "sMrf", "sMrt", "sMtf"), 2, sim
  # apply to p1 too
```

```

p1pairs <- tibble::as_tibble_row(mod$mean$p1) %>%
  pivot_coordpairs(colpairs = colpairs)

# apply to G0 too
# first get start and end location of pretty axes around G01
arrowends <- t(t(mod$G0[, -1] - mod$G0[, 1]) * mod$a[-1]/10) + mod$G0[, 1] # convert to differ
colnames(arrowends) <- paste0("G0", 1+ (1:ncol(arrowends)))

axisarrows <- lapply(1:nrow(mod$pred), function(idx){
  pred <- mod$pred[idx, ]
  # rotate (parallel transport) arrows to be around predicted mean
  arrowends <- rotationmat_amaral(mod$G0[, 1], pred) %*% arrowends
  # include start location too
  names(pred) <- paste0("start", rownames(arrowends))
  as_tibble(t(arrowends), rownames = "Axis") %>%
    bind_cols(t(pred)) %>%
    bind_cols(extra[idx, ])
}) %>%
  bind_rows()
# apply orthogonal projections
axisarrows_pairs <- lapply(colpairs, function(pair) {
  axisarrows %>%
    select(everything(), -starts_with("s"), -starts_with("starts"), all_of(pair), all_of(p
    rename(A = last_col(3), B = last_col(2), startA = last_col(1), startB = last_col(0)) %>%
    mutate(pair1=pair[1],
           pair2=pair[2],
           pair = paste(pair, collapse = "-"))
}) %>%
  bind_rows()

# old G0 axes
colnames(mod$G0) <- paste0("G0", 1:ncol(mod$G0))
G0pairs <- as_tibble(t(mod$G0), rownames = "Axis") %>%
  pivot_coordpairs(colpairs = colpairs)

predsobs <- bind_cols(mod$pred %>%
  as_tibble() %>%
  rename_with(~paste0("p_", .)),
  mod$y,
  extra)
pair_dfs <- lapply(colpairs, function(pair) {
  predsobs %>%

```

```

    select(everything(), -starts_with("s"), -starts_with("p_s"), all_of(pair), all_of(paste0(pair, "s"))) %>%
    rename(A = last_col(3), B = last_col(2), p_A = last_col(1), p_B = last_col(0)) %>%
    mutate(pair1=pair[1],
           pair2=pair[2],
           pair = paste(pair, collapse = "-"))
  })
pairsdf <- bind_rows(pair_dfs)
attr(pairsdf, "p1") <- p1pairs
attr(pairsdf, "G0") <- G0pairs
attr(pairsdf, "Garrows") <- axisarrows_pairs
attr(pairsdf, "coordnames") <- c("s1", "s2", "sMrt", "sMrf", "sMtf")
pairsdf
}

```

```

get_predobspairsdf_nat(mod_SvMF, s4df_clean %>% select(-starts_with("s"))) %>%
  pairedplotggprep() +
  geom_segment(aes(x=p_A, y=p_B, xend=A, yend=B, col = Longitude),
              alpha = 0.5,
              arrow = grid::arrow(length = unit(0.02, "npc"))) +
  geom_point(aes(x=p_A, y=p_B, fill = Longitude),
            size = 1.5,
            shape = 21) +
  geom_point(aes(x=A, y=B), size = 2, col = "blue",
            shape = 4,
            data = attr(get_predobspairsdf_nat(mod_SvMF), "p1")) +
  scale_fill_viridis_c() +
  scale_color_viridis_c() +
  ggtitle("Predictions")

```

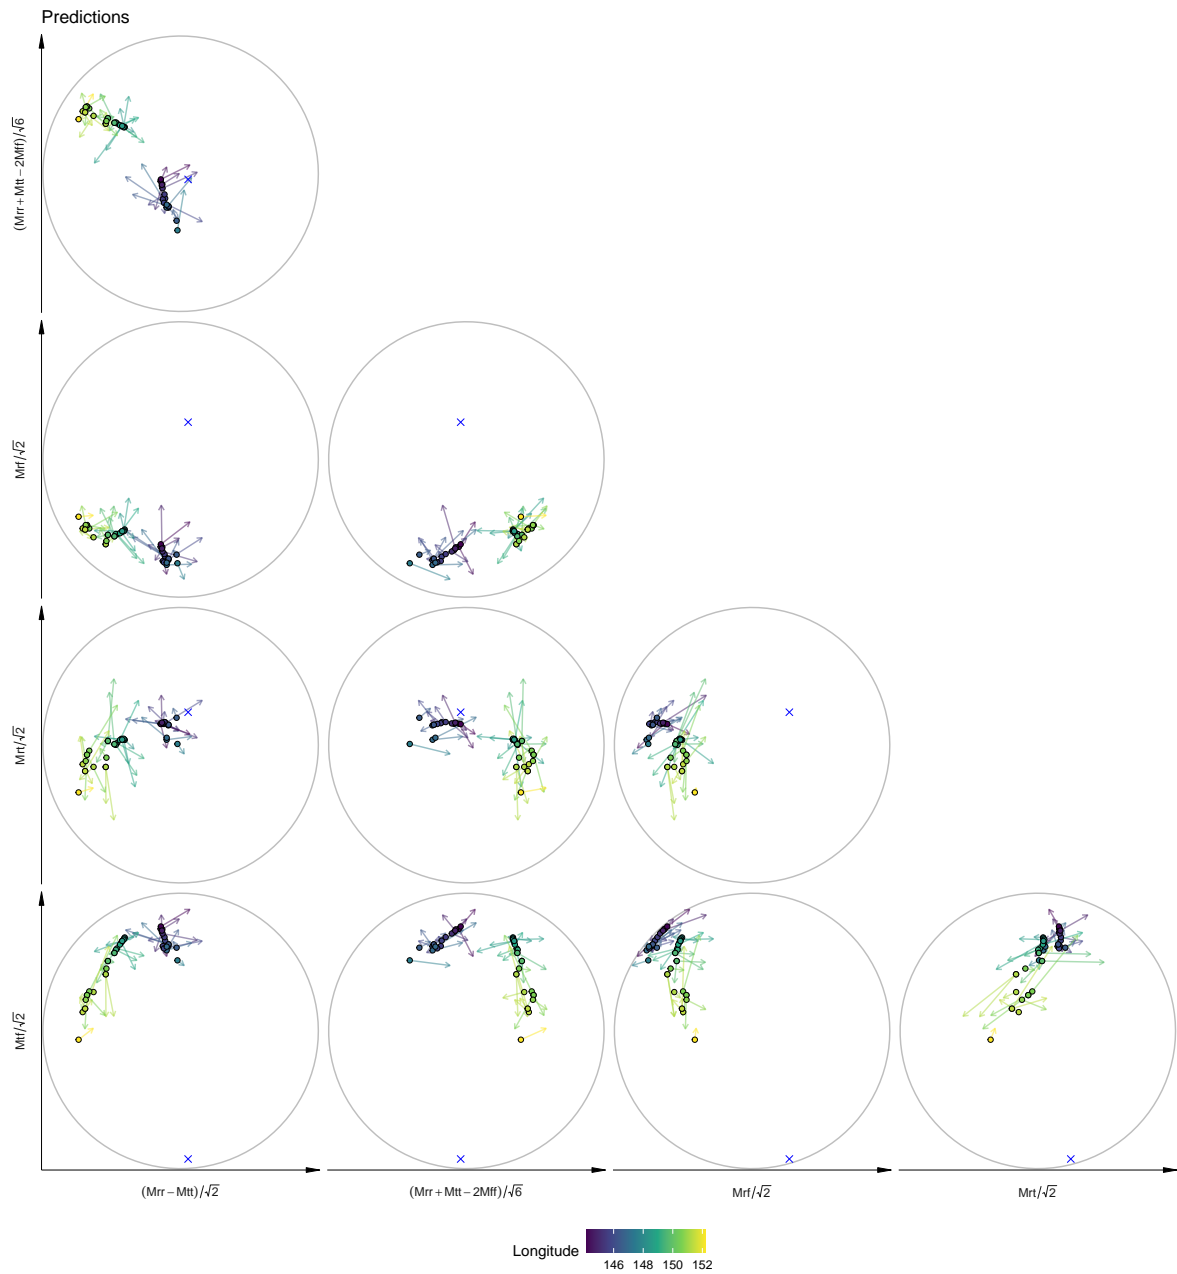

```
ggsave("earthq_predictions.pdf", width = 12, height = 13)
```

## 6 Main Figure: Observed and Predicted

```

obsplots <- get_predobspairsdf_nat(mod_SvMF, s4df_clean %>% select(-starts_with("s")),
                                   colpairs = strsplit(c("s1-s2", "sMtf-s2", "sMrt-s2"), "-")) %>%
  pairedplotggprep() +
  geom_point(aes(x=A, y=B, col = Longitude), size = 1) +
  scale_color_viridis_c() +
  theme(plot.margin = unit(c(0,2,0,2), "mm"),
        axis.line.y = element_line(arrow = grid::arrow(type = "closed", angle = 10, length = unit(0.2),
                                                         linewidth = 0.2),
                                     strip.text = element_text(margin = margin(0, 0, 0, 0), size = 8),
                                     strip.text.x.bottom = element_blank(),
                                     legend.position = "right")

pairedddf <- get_predobspairsdf_nat(mod_SvMF, s4df_clean %>% select(-starts_with("s")),
                                   colpairs = strsplit(c("s1-s2", "sMtf-s2", "sMrt-s2"), "-"))
predplots <- pairedddf %>%
  pairedplotggprep() +
  geom_segment(aes(x=p_A, y=p_B, xend=A, yend=B, col = Longitude),
              alpha = 1,
              arrow = grid::arrow(length = unit(0.02, "npc")))) +
  geom_point(aes(x=p_A, y=p_B, fill = Longitude),
            size = 1.5,
            shape = 21) +
  geom_point(aes(x=A, y=B), size = 2, col = "blue",
            shape = 21,
            data = ~attr(pairedddf, "G0") %>% filter(Axis == "G01") %>% filter(pair %in% .x$pair)) +
  geom_point(aes(x=A, y=B), size = 2, col = "blue",
            shape = 4,
            data = ~(attr(pairedddf, "p1") %>% filter(pair %in% .x$pair))
            ) +
  scale_color_viridis_c() +
  scale_fill_viridis_c() +
  theme(plot.margin = unit(c(0,2,0,2), "mm"),
        axis.line = element_line(arrow = grid::arrow(type = "closed", angle = 10, length = unit(0.2),
                                                         linewidth = 0.2),
                                     strip.text = element_text(margin = margin(0, 0, 0, 0), size = 8),
                                     legend.position = "right")

obsplots/
predplots +

```

```
plot_layout(guides = "collect")
```

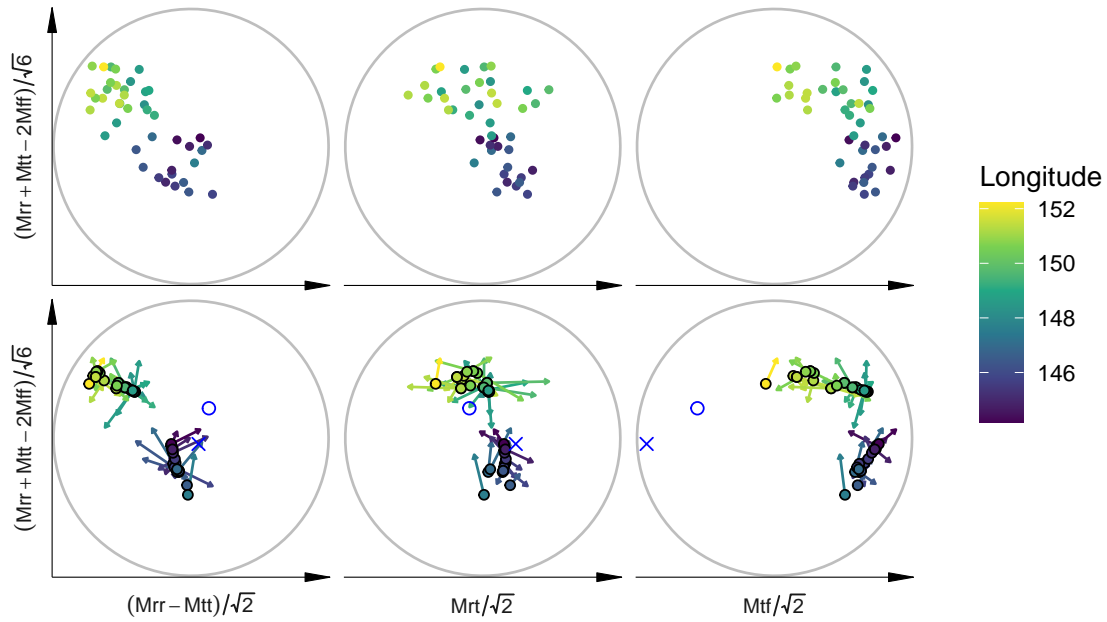

```
ggsave("earthquake_results.pdf", width = 7, height = 4)
```

## 7 Angles to $b_{01}$ and $\gamma_{01}$

The range of the angle between predicted mean and estimated  $b_{01}$  is:

```
range(acos(mod_SvMF$pred %*% mod_SvMF$mean$p1))
```

```
[1] 1.763871 2.570258
```

The range of the angle between predicted mean and estimated  $\gamma_{01}$  is:

```
range(acos(mod_SvMF$pred %*% mod_SvMF$G0[,1]))
```

```
[1] 1.839712 3.065784
```

## 8 Predictions in Standardised Coordinates

Below I plot the predictions in standardised coordinates. In the first plot the residuals are coloured arrows and the orientation axes for each prediction are shown in grey. In the second plot the residuals are still coloured arrows, but the orientation axes are shown as strong blued, red, purple etc lines.

```
get_predobspairsdf <- function(mod,
                                extra = NULL,
                                colpairs = combn(paste0("Y",1:5), 2, simplify = FALSE),
                                useG0 = FALSE){

  # standard rotations
  if (useG0){
    ystd <- standardise_sph(mod$y, tG = t(mod$G0))
  } else {
    ystd <- standardise_sph(mod$y)
  }

  colnames(ystd) <- paste0("Y", 1:ncol(ystd))
  predstd <- standardise_sph(mod$pred, attr(ystd, "std_rotation"))
  colnames(predstd) <- paste0("p_Y", 1:ncol(predstd))
  # apply to p1 too
  p1std <- standardise_sph(matrix(mod$mean$p1, nrow = 1), attr(ystd, "std_rotation"))
  colnames(p1std) <- paste0("Y", 1:ncol(ystd))
  p1pairs <- as_tibble(p1std) %>%
    pivot_coordpairs(colpairs = colpairs)
  # apply to G0 too
  # first get start and end location of pretty axes around G01
  arrowends <- t(t(mod$G0[,-1] - mod$G0[,1]) * mod$a[-1]/10) + mod$G0[,1] # convert to differ
  colnames(arrowends) <- paste0("G0", 1+ (1:ncol(arrowends)))

  axisarrows <- lapply(1:nrow(mod$pred), function(idx){
    pred <- mod$pred[idx, ]
    # rotate (parallel transport) arrows to be around predicted mean, then rotate again for s
    stdarrowends <- attr(ystd, "std_rotation") %*% rotationmat_amaral(mod$G0[,1], pred) %*% a
    rownames(stdarrowends) <- paste0("Y", 1:ncol(ystd))
    # include start location too
    stdpred <- drop(attr(ystd, "std_rotation") %*% pred)
    names(stdpred) <- paste0("start", rownames(stdarrowends))
    as_tibble(t(stdarrowends), rownames = "Axis") %>%
      bind_cols(t(stdpred)) %>%
      bind_cols(extra[idx, ])
```

```

}) %>%
  bind_rows()
# apply orthogonal projections
axisarrows_pairs <- lapply(colpairs, function(pair) {
  axisarrows %>%
    select(everything(), -starts_with("Y"), -starts_with("startY"), all_of(pair), all_of(p
    rename(A = last_col(3), B = last_col(2), startA = last_col(1), startB = last_col(0)) %>%
    mutate(pair1=pair[1],
           pair2=pair[2],
           pair = paste(pair, collapse = "-"))
}) %>%
  bind_rows()

# old G0 axes
G0std <- attr(ystd, "std_rotation") %*% mod$G0
rownames(G0std) <- paste0("Y", 1:ncol(ystd))
colnames(G0std) <- paste0("G0", 1:ncol(G0std))
G0pairs <- as_tibble(t(G0std), rownames = "Axis") %>%
  pivot_coordpairs(colpairs = colpairs)

predsobs <- bind_cols(predstd,
                      ystd,
                      extra)
pair_dfs <- lapply(colpairs, function(pair) {
  predsobs %>%
    select(everything(), -starts_with("Y"), -starts_with("p_Y"), all_of(pair), all_of(paste
    rename(A = last_col(3), B = last_col(2), p_A = last_col(1), p_B = last_col(0)) %>%
    mutate(pair1=pair[1],
           pair2=pair[2],
           pair = paste(pair, collapse = "-"))
})
pairsdf <- bind_rows(pair_dfs)
attr(pairsdf, "p1") <- p1pairs
attr(pairsdf, "G0") <- G0pairs
attr(pairsdf, "Garrows") <- axisarrows_pairs
attr(pairsdf, "coordnames") <- paste0("Y", 1:5)
pairsdf
}

```

```

getG0arrows <- function(mod_SvMF){
  names(mod_SvMF$a) <- paste0("G0", 1:length(mod_SvMF$a))
  tibble::enframe(mod_SvMF$a, name = "Axis", value = "scale")
}

```



```

orientations <- get_predobspairsdf(mod_SvMF) %>%
  attr("G0") %>%
  left_join(tibble::enframe(mod_SvMF$a, name = "Axis", value = "scale"), by = "Axis") %>%
  # mutate(across(c(A, B, starts_with("Y")), ~case_when(Axis != "G01" ~ .x * scale/20, TRUE ~ .x)) %>%
  group_by(pair) %>%
  arrange(Axis) %>%
  select(-starts_with("Y")) %>%
  mutate(
    Astart = first(A),
    Bstart = first(B),
    A = A - Astart,
    B = B - Bstart) %>% #make everything vectors - works because projection orthogonal
  # across(c(A, B), ~.x - first(.x))) %>% #make everything vectors - works because projection orthogonal
  mutate(across(c(A, B), ~.x * scale/10)) %>% #scale axes by their estimated scale (G01 is not scaled)
  filter(Axis != "G01") %>%
  ungroup() %>%
  # add G01 back into A B etc
  mutate(A = A + Astart, B = B + Bstart)
return(orientations)
}

```

```

defaultplot_pred <- function(mod_SvMF, s4df_clean, focusaxes = FALSE, focusresponse = FALSE){
  plotobj <- get_predobspairsdf(mod_SvMF, bind_cols(s4df_clean, rdist = mod_SvMF$dists, rename(dists, "G01")))
  pairedplotggprep()
  if (!focusaxes){
    plotobj <- plotobj %>%
      addaxes(mod_SvMF, axiscolour = rep("grey", 4), alpha = 0.5)
  }
  if (focusresponse){
    plotobj <- plotobj +
      geom_point(aes(x=A, y=B, col = Longitude), size = 2)
  } else {
    plotobj <- plotobj +
      geom_point(aes(x=p_A, y=p_B, col = Longitude), size = 2)
  }
  plotobj <- plotobj +
    geom_point(aes(x=A, y=B), size = 2, col = "blue",
      data = attr(get_predobspairsdf(mod_SvMF), "p1")) +
    geom_point(aes(x=-A, y=-B), size = 2, col = "blue", shape = 21,
      data = attr(get_predobspairsdf(mod_SvMF), "p1")) +
    geom_point(aes(x=A, y=B), size = 2, col = "red",
      data = attr(get_predobspairsdf(mod_SvMF), "G0") %>% filter(Axis == "G01")) +

```

```

geom_segment(aes(x=Astart,y=Bstart, xend=A, yend=B),
             data = getG0arrows(mod_SvMF) %>% filter(Axis == "G02"),
             arrow = grid::arrow(length = unit(0.02, "npc")))) +
geom_segment(aes(x=Astart,y=Bstart, xend=A, yend=B),
             col = "grey",
             data = getG0arrows(mod_SvMF) %>% filter(Axis == "G03"),
             arrow = grid::arrow(length = unit(0.02, "npc")))) +
geom_point(aes(x=-A, y=-B), size = 2, col = "red", shape = 21,
           data = attr(get_predobspairsdf(mod_SvMF), "G0") %>% filter(Axis == "G01")) +
geom_segment(aes(x=p_A, y=p_B, xend=A, yend=B, col = Longitude),
             alpha = 0.5,
             arrow = grid::arrow(length = unit(0.02, "npc")))) +
scale_color_viridis_c() +
ggtitle("Prediction Highlighted")
if (focusaxes){
  plotobj <- plotobj %>%
    addaxes(mod_SvMF, axiscolour = c("red", "green", "blue", "purple"))
}
return(plotobj)
}

addaxes <- function(plotobj, mod_SvMF, axiscolour = c("red", "green", "blue", "purple"), alpha)
plotobj +
  geom_segment(aes(x=startA,y=startB, xend=A, yend=B),
               data = attr(get_predobspairsdf(mod_SvMF), "Garrows") %>% filter(Axis == "G01"),
               alpha = alpha,
               col = axiscolour[1]) +
  # arrow = grid::arrow(length = unit(0.02, "npc"), type = "closed")) +
  geom_segment(aes(x=startA,y=startB, xend=A, yend=B),
               data = attr(get_predobspairsdf(mod_SvMF), "Garrows") %>% filter(Axis == "G02"),
               alpha = alpha,
               col = axiscolour[2]) +
  # arrow = grid::arrow(length = unit(0.02, "npc"), type = "closed")) +
  geom_segment(aes(x=startA,y=startB, xend=A, yend=B),
               data = attr(get_predobspairsdf(mod_SvMF), "Garrows") %>% filter(Axis == "G03"),
               alpha = alpha,
               col = axiscolour[3]) +
  # arrow = grid::arrow(length = unit(0.02, "npc"), type = "closed")) +
  geom_segment(aes(x=startA,y=startB, xend=A, yend=B),
               data = attr(get_predobspairsdf(mod_SvMF), "Garrows") %>% filter(Axis == "G04"),
               alpha = alpha,
               col = axiscolour[4])
  # arrow = grid::arrow(length = unit(0.02, "npc"), type = "closed"))

```

```
}
defaultplot_pred(mod_SvMF, s4df_clean)
```

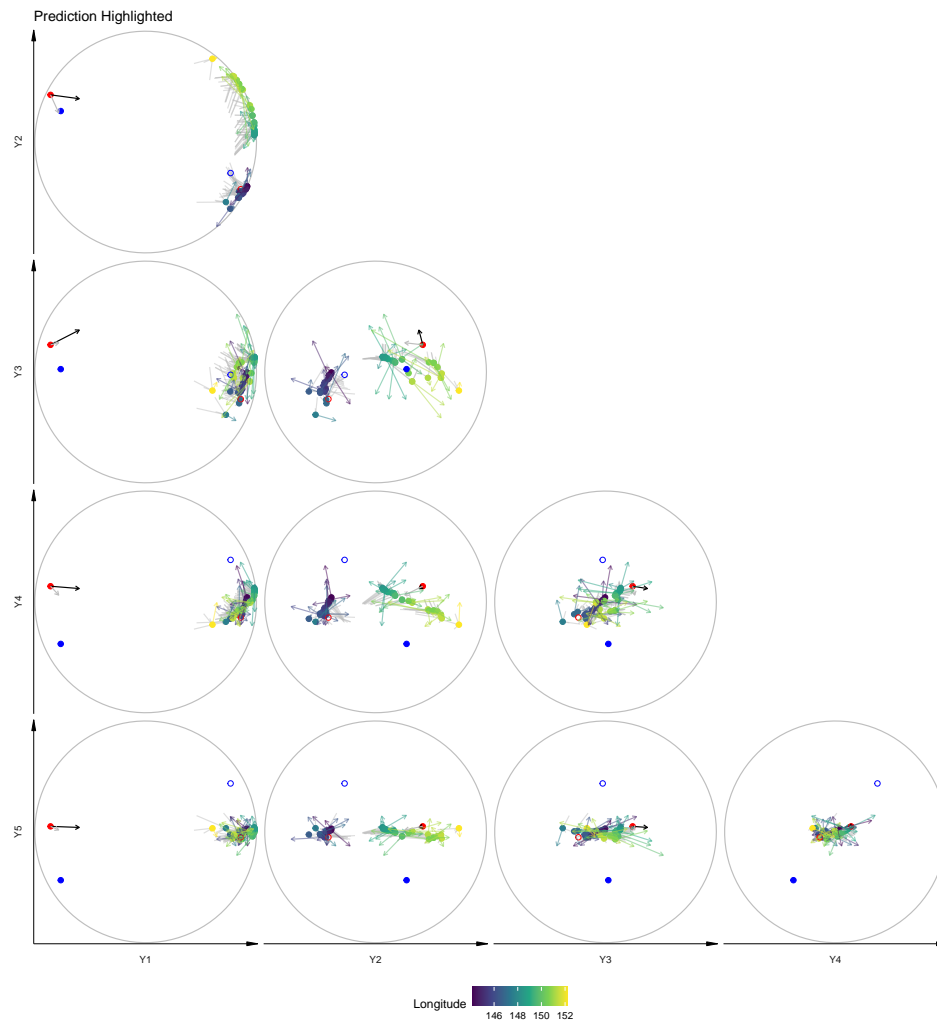

```
defaultplot_pred(mod_SvMF, s4df_clean, focusaxes = TRUE)
```

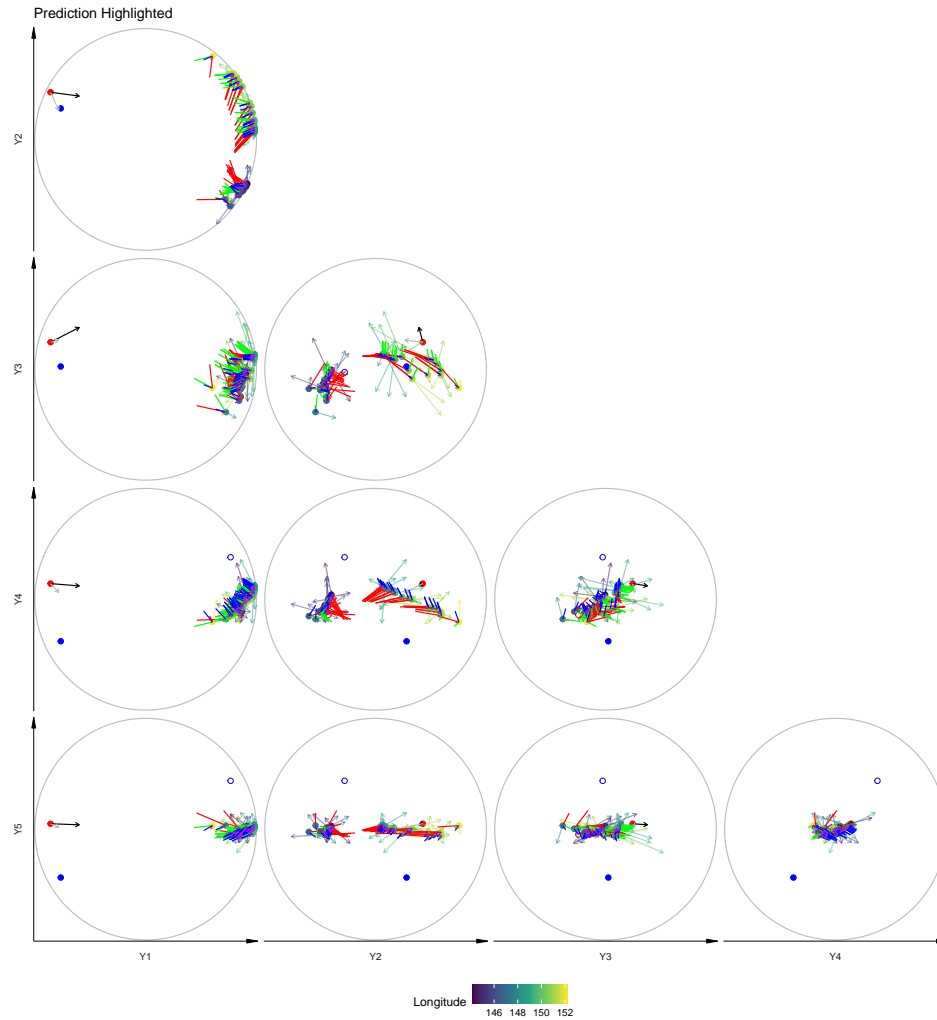

## 9 Model Diagnostics

### 9.1 Rotated Residuals (SI Figure)

Here we plot the rotated residuals against each of the axes defined by  $\Gamma_0$ . We can see the ellipsoidal nature of Scaled von Mises Fisher residuals. The maximum size of a rotated residual is 1 (grey circular boundary).

```
mod_SvMF$rresids_G0 %>%
  as_tibble() %>%
  bind_cols(s4df_clean, rdist = mod_SvMF$dists) %>%
```

```

bind_cols(rename_with(as_tibble(mod_SvMF$rresids_std), ~paste0("std", .x))) %>%
pivot_coordpairs(coordnames = paste0("r", 1:4)) %>%
pairedplotggprep() +
stat_summary_2d(fun = mean,
                aes(z = Longitude, fill = after_stat(value)),
                bins = 10) +
geom_point(aes(fill = Longitude), size = 2, shape = 21) +
scale_fill_viridis_c(name = "Longitude") +
scale_color_viridis_c(name = "Longitude")

```

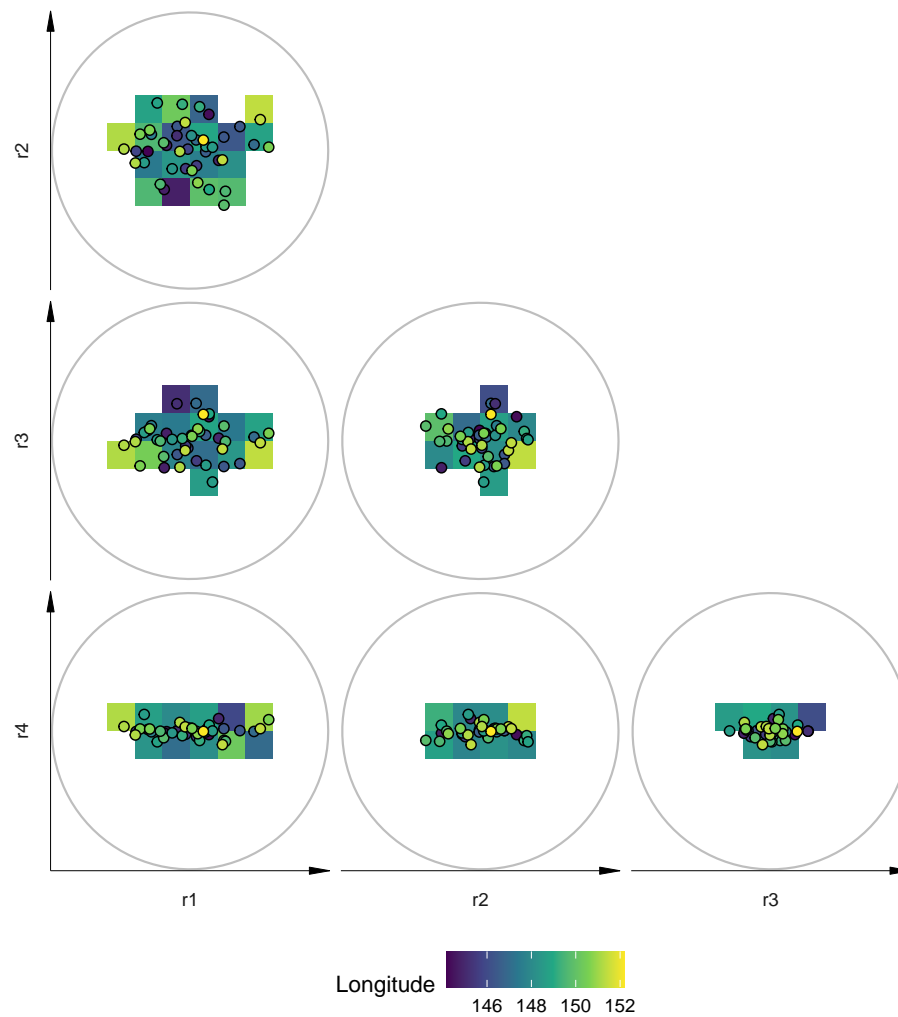

```

ggsave("earthq_rresids.pdf", width = 8, height = 7)

```

## 9.2 Residual Mean by Covariates (SI Figure)

Below is the residuals in each of the basis coordinates given by the SvMF orientation against covariate values.

```
bind_cols(mod_SvMF$resids_GO, s4df_clean) %>%
  st_drop_geometry() %>%
  tidyr::pivot_longer(matches("^r.$"), names_to = "raxis", values_to = "value") %>%
  tidyr::pivot_longer(c(Latitude, Longitude, fstrike, dist, Depth), names_to = "covariate", v
  filter(!(covariate == "dist" & (cvalue > 50000))) %>%
  ggplot(aes(x = cvalue, y = value)) +
  facet_grid(rows = vars(raxis), cols = vars(covariate), scales = "free",
               labeller = as_labeller(c(Depth = "Depth", dist = "Distance", fstrike = "Strike"
                                         r1 = "r1", r2 = "r2", r3 = "r3", r4 = "r4")))) +
  geom_hline(yintercept = 0, col = "blue", lty = "dashed") +
  geom_smooth(method = "loess", formula = 'y ~ x', data = ~filter(.x, covariate != "Depth"))
  geom_point() +
  stat_summary(fun.data = mean_se, geom = "errorbar", width = 1.5, col = "blue", data = ~fil
  scale_y_continuous(name = "Residual") +
  scale_x_continuous(name = "Covariate Value")
```

```
Warning in simpleLoess(y, x, w, span, degree = degree, parametric = parametric,
: pseudoinverse used at -3.4
```

```
Warning in simpleLoess(y, x, w, span, degree = degree, parametric = parametric,
: neighborhood radius 0.2
```

```
Warning in simpleLoess(y, x, w, span, degree = degree, parametric = parametric,
: reciprocal condition number 7.3434e-17
```

```
Warning in predLoess(object$y, object$x, newx = if (is.null(newdata)) object$x
else if (is.data.frame(newdata))
as.matrix(model.frame(delete.response(terms(object))), : pseudoinverse used at
-3.4
```

```
Warning in predLoess(object$y, object$x, newx = if (is.null(newdata)) object$x
else if (is.data.frame(newdata))
as.matrix(model.frame(delete.response(terms(object))), : neighborhood radius 0.2
```

Warning in predLoess(object\$y, object\$x, newx = if (is.null(newdata)) object\$x  
else if (is.data.frame(newdata))  
as.matrix(model.frame(delete.response(terms(object))), : reciprocal condition  
number 7.3434e-17

Warning in simpleLoess(y, x, w, span, degree = degree, parametric = parametric,  
: pseudoinverse used at -3.4

Warning in simpleLoess(y, x, w, span, degree = degree, parametric = parametric,  
: neighborhood radius 0.2

Warning in simpleLoess(y, x, w, span, degree = degree, parametric = parametric,  
: reciprocal condition number 7.3434e-17

Warning in predLoess(object\$y, object\$x, newx = if (is.null(newdata)) object\$x  
else if (is.data.frame(newdata))  
as.matrix(model.frame(delete.response(terms(object))), : pseudoinverse used at  
-3.4

Warning in predLoess(object\$y, object\$x, newx = if (is.null(newdata)) object\$x  
else if (is.data.frame(newdata))  
as.matrix(model.frame(delete.response(terms(object))), : neighborhood radius 0.2

Warning in predLoess(object\$y, object\$x, newx = if (is.null(newdata)) object\$x  
else if (is.data.frame(newdata))  
as.matrix(model.frame(delete.response(terms(object))), : reciprocal condition  
number 7.3434e-17

Warning in simpleLoess(y, x, w, span, degree = degree, parametric = parametric,  
: pseudoinverse used at -3.4

Warning in simpleLoess(y, x, w, span, degree = degree, parametric = parametric,  
: neighborhood radius 0.2

Warning in simpleLoess(y, x, w, span, degree = degree, parametric = parametric,  
: reciprocal condition number 7.3434e-17

Warning in predLoess(object\$y, object\$x, newx = if (is.null(newdata)) object\$x  
else if (is.data.frame(newdata))  
as.matrix(model.frame(delete.response(terms(object))), : pseudoinverse used at  
-3.4

```
Warning in predLoess(object$y, object$x, newx = if (is.null(newdata)) object$x
else if (is.data.frame(newdata))
as.matrix(model.frame(delete.response(terms(object))), : neighborhood radius 0.2
```

```
Warning in predLoess(object$y, object$x, newx = if (is.null(newdata)) object$x
else if (is.data.frame(newdata))
as.matrix(model.frame(delete.response(terms(object))), : reciprocal condition
number 7.3434e-17
```

```
Warning in simpleLoess(y, x, w, span, degree = degree, parametric = parametric,
: pseudoinverse used at -3.4
```

```
Warning in simpleLoess(y, x, w, span, degree = degree, parametric = parametric,
: neighborhood radius 0.2
```

```
Warning in simpleLoess(y, x, w, span, degree = degree, parametric = parametric,
: reciprocal condition number 7.3434e-17
```

```
Warning in predLoess(object$y, object$x, newx = if (is.null(newdata)) object$x
else if (is.data.frame(newdata))
as.matrix(model.frame(delete.response(terms(object))), : pseudoinverse used at
-3.4
```

```
Warning in predLoess(object$y, object$x, newx = if (is.null(newdata)) object$x
else if (is.data.frame(newdata))
as.matrix(model.frame(delete.response(terms(object))), : neighborhood radius 0.2
```

```
Warning in predLoess(object$y, object$x, newx = if (is.null(newdata)) object$x
else if (is.data.frame(newdata))
as.matrix(model.frame(delete.response(terms(object))), : reciprocal condition
number 7.3434e-17
```



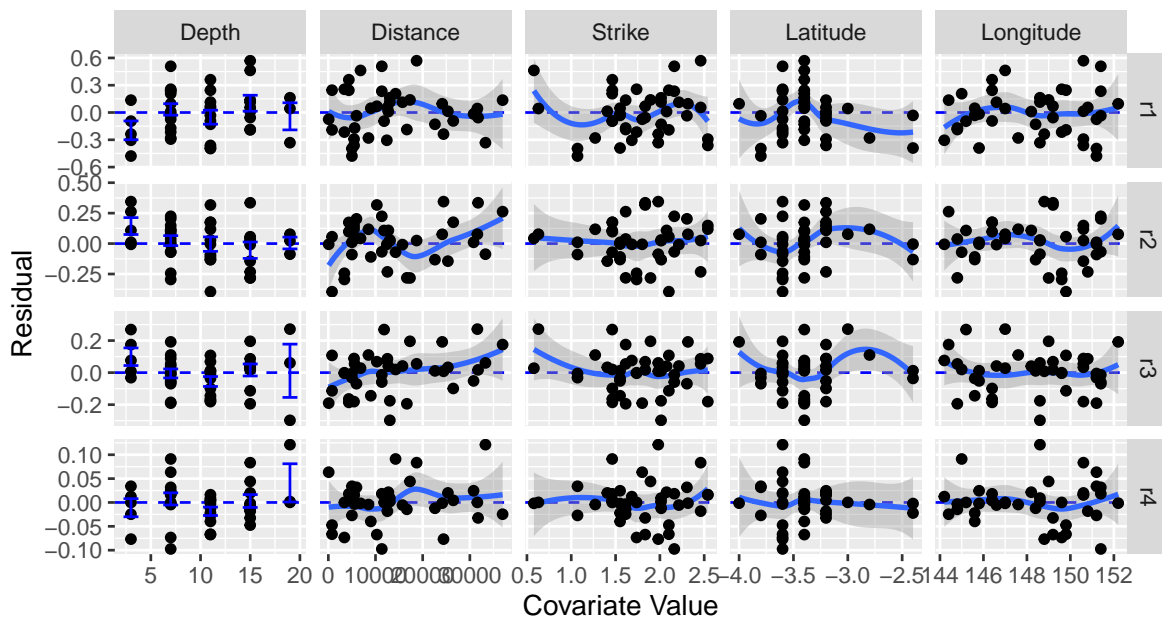

```
ggsave("earthq_rresids2.pdf", width = 8, height = 6)
```

```
Warning in simpleLoess(y, x, w, span, degree = degree, parametric = parametric,
: pseudoinverse used at -3.4
```

```
Warning in simpleLoess(y, x, w, span, degree = degree, parametric = parametric,
: neighborhood radius 0.2
```

```
Warning in simpleLoess(y, x, w, span, degree = degree, parametric = parametric,
: reciprocal condition number 7.3434e-17
```

```
Warning in predLoess(object$y, object$x, newx = if (is.null(newdata)) object$x
else if (is.data.frame(newdata))
as.matrix(model.frame(delete.response(terms(object))), : pseudoinverse used at
-3.4
```

```
Warning in predLoess(object$y, object$x, newx = if (is.null(newdata)) object$x
else if (is.data.frame(newdata))
as.matrix(model.frame(delete.response(terms(object))), : neighborhood radius 0.2
```

Warning in predLoess(object\$y, object\$x, newx = if (is.null(newdata)) object\$x  
else if (is.data.frame(newdata))  
as.matrix(model.frame(delete.response(terms(object))), : reciprocal condition  
number 7.3434e-17

Warning in simpleLoess(y, x, w, span, degree = degree, parametric = parametric,  
: pseudoinverse used at -3.4

Warning in simpleLoess(y, x, w, span, degree = degree, parametric = parametric,  
: neighborhood radius 0.2

Warning in simpleLoess(y, x, w, span, degree = degree, parametric = parametric,  
: reciprocal condition number 7.3434e-17

Warning in predLoess(object\$y, object\$x, newx = if (is.null(newdata)) object\$x  
else if (is.data.frame(newdata))  
as.matrix(model.frame(delete.response(terms(object))), : pseudoinverse used at  
-3.4

Warning in predLoess(object\$y, object\$x, newx = if (is.null(newdata)) object\$x  
else if (is.data.frame(newdata))  
as.matrix(model.frame(delete.response(terms(object))), : neighborhood radius 0.2

Warning in predLoess(object\$y, object\$x, newx = if (is.null(newdata)) object\$x  
else if (is.data.frame(newdata))  
as.matrix(model.frame(delete.response(terms(object))), : reciprocal condition  
number 7.3434e-17

Warning in simpleLoess(y, x, w, span, degree = degree, parametric = parametric,  
: pseudoinverse used at -3.4

Warning in simpleLoess(y, x, w, span, degree = degree, parametric = parametric,  
: neighborhood radius 0.2

Warning in simpleLoess(y, x, w, span, degree = degree, parametric = parametric,  
: reciprocal condition number 7.3434e-17

Warning in predLoess(object\$y, object\$x, newx = if (is.null(newdata)) object\$x  
else if (is.data.frame(newdata))  
as.matrix(model.frame(delete.response(terms(object))), : pseudoinverse used at  
-3.4

```
Warning in predLoess(object$y, object$x, newx = if (is.null(newdata)) object$x
else if (is.data.frame(newdata))
as.matrix(model.frame(delete.response(terms(object))), : neighborhood radius 0.2
```

```
Warning in predLoess(object$y, object$x, newx = if (is.null(newdata)) object$x
else if (is.data.frame(newdata))
as.matrix(model.frame(delete.response(terms(object))), : reciprocal condition
number 7.3434e-17
```

```
Warning in simpleLoess(y, x, w, span, degree = degree, parametric = parametric,
: pseudoinverse used at -3.4
```

```
Warning in simpleLoess(y, x, w, span, degree = degree, parametric = parametric,
: neighborhood radius 0.2
```

```
Warning in simpleLoess(y, x, w, span, degree = degree, parametric = parametric,
: reciprocal condition number 7.3434e-17
```

```
Warning in predLoess(object$y, object$x, newx = if (is.null(newdata)) object$x
else if (is.data.frame(newdata))
as.matrix(model.frame(delete.response(terms(object))), : pseudoinverse used at
-3.4
```

```
Warning in predLoess(object$y, object$x, newx = if (is.null(newdata)) object$x
else if (is.data.frame(newdata))
as.matrix(model.frame(delete.response(terms(object))), : neighborhood radius 0.2
```

```
Warning in predLoess(object$y, object$x, newx = if (is.null(newdata)) object$x
else if (is.data.frame(newdata))
as.matrix(model.frame(delete.response(terms(object))), : reciprocal condition
number 7.3434e-17
```

### 9.3 Standardised Residuals

Below the same residuals are transformed using the estimated concentration and Scale von Mises Fisher scales so that, at high-concentrations, the residuals should be close to a standard multivariate Normal (Scealy and Wood, 2019, Proposition 2).

```

mod_SvMF$rresids_std %>%
  as_tibble() %>%
  bind_cols(s4df_clean, rdist = mod_SvMF$dists) %>%
  pivot_coordpairs(coordnames = paste0("r", 1:4)) %>%
  ggplot(mapping = aes(x=A, y=B, col = fstrike)) +
  facet_wrap(vars(pair2, pair1)) +
  theme(strip.text.y = element_text(angle = 90),
        strip.placement = "outside",
        axis.title = element_blank(),
        strip.background = element_blank()) +
  geom_hline(yintercept = 0, lty = "dashed") +
  geom_vline(xintercept = 0, lty = "dashed") +
  geom_point(size = 1) +
  scale_color_viridis_c() +
  coord_fixed()

```

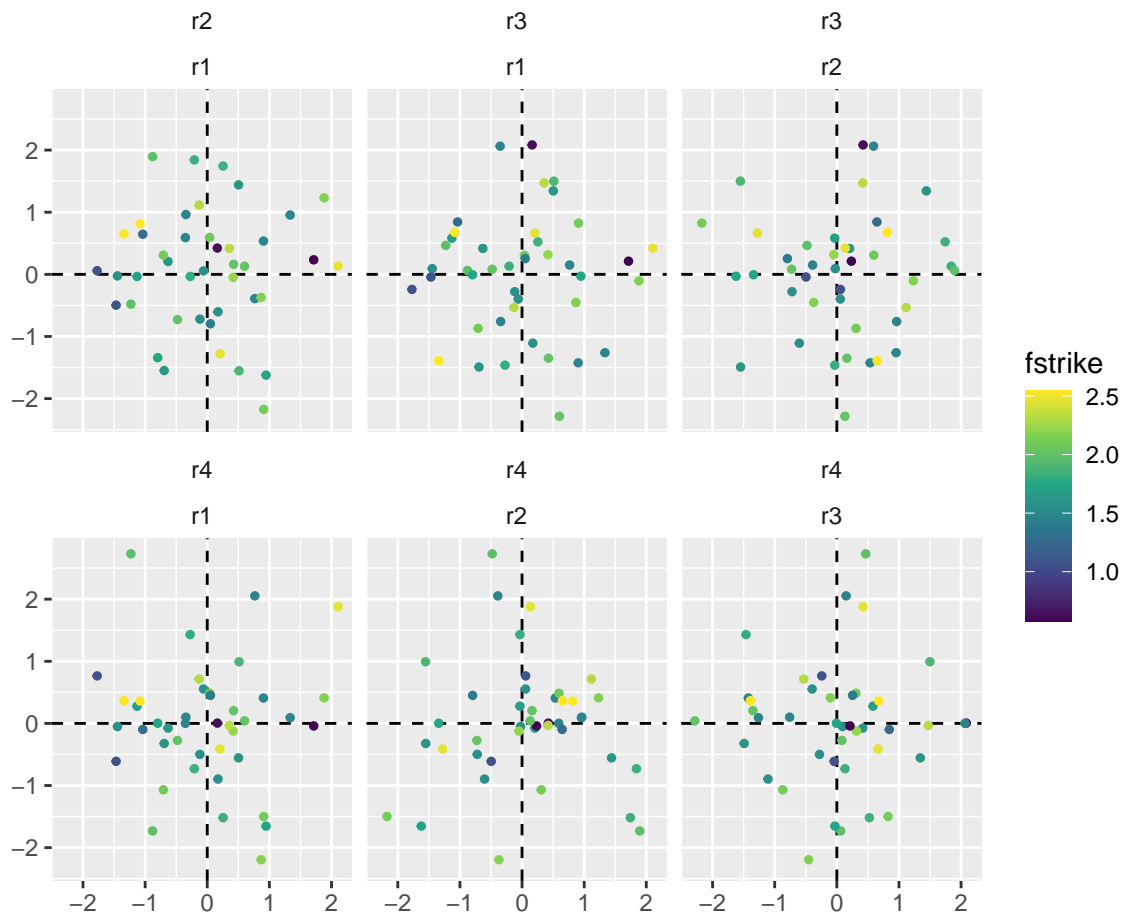

#### 9.4 Standardised Residual Distance (SI Figure)

```
stdrdist <- sqrt(rowSums(mod_SvMF$rresids_std^2))
stdrdist[!attr(mod_SvMF$rresids_std, "samehemisphere")] <- NA_real_
p1 <- bind_cols(srdist = stdrdist, rdists = mod_SvMF$dists, s4df_clean) %>%
  bind_cols(rename_with(as_tibble(mod_SvMF$rresids_std), ~paste0("std", .x))) %>%
  ggplot(aes(y=srdist, x = Longitude)) +
  geom_point() +
  ylab("Scaled Residual\nDistance")

p2 <- bind_cols(srdist = stdrdist, rdists = mod_SvMF$dists, s4df_clean) %>%
  bind_cols(rename_with(as_tibble(mod_SvMF$rresids_std), ~paste0("std", .x))) %>%
  ggplot(aes(y=srdist, x = fstrike)) +
```

```
geom_point() +
ylab("Scaled Residual\nDistance") +
xlab("Strike")

p1 + p2 + plot_layout(axes = "collect")
```

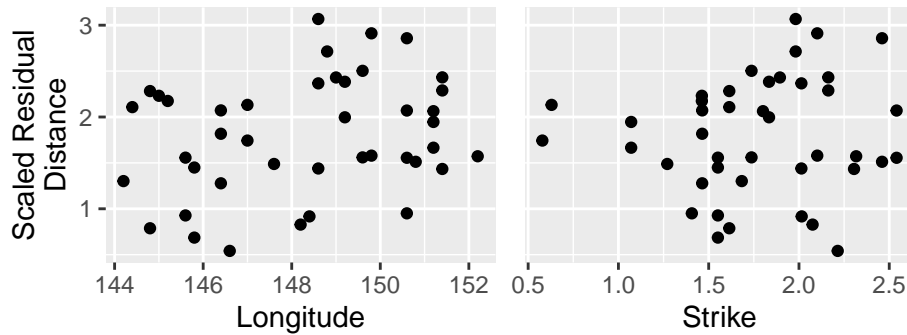

```
ggsave("earthq_srdist.pdf", width = 5, height = 2)
```

## 9.5 Residual Distance (Unstandardised)

```
p1 <- bind_cols(rdist = mod_SvMF$dists, s4df_clean) %>%
  bind_cols(rename_with(as_tibble(mod_SvMF$rresids_std), ~paste0("std", .x))) %>%
  ggplot(aes(y=rdist, x = Longitude)) +
  geom_point()

p2 <- bind_cols(rdist = mod_SvMF$dists, s4df_clean) %>%
  bind_cols(rename_with(as_tibble(mod_SvMF$rresids_std), ~paste0("std", .x))) %>%
  ggplot(aes(y=rdist, x = fstrike)) +
  geom_point()

p1 + p2
```

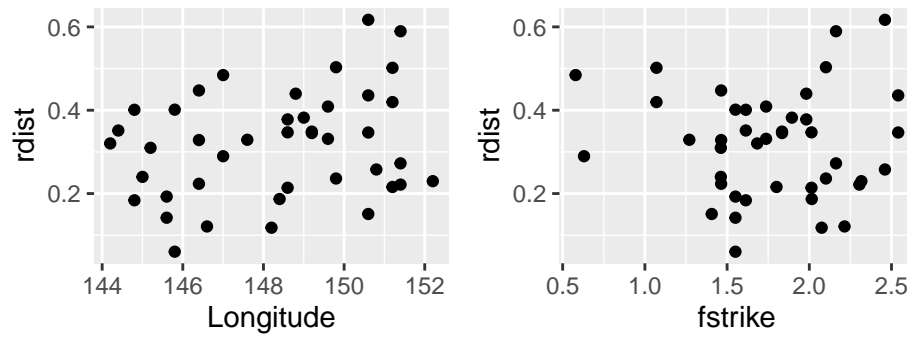

## 10 Likelihood Ratio Test of vMF vs SvMF

First get best vMF model

```
mod_vMF <- mobius_vMF(y = mod_SvMF$y,
                      xs = NULL,
                      xe = mod_SvMF$xe,
                      type = "LinEuc")
mod_vMF_restarts <- pbapply::pblapply(1:100, function(seed){mobius_vMF_restart(mod_vMF, seed,
```

Warning in mobius\_vMF(y = mod\_vMF\$y, xs = mod\_vMF\$xs, xe = mod\_vMF\$xe, fix\_qs1 = mod\_vMF\$linktype\$fix\_qs1, : NLOPT\_MAXEVAL\_REACHED: Optimization stopped because maxeval (above) was reached.

```
lapply(mod_vMF_restarts, "[", "AIC") %>%
  unlist() %>%
  tibble::enframe("seed", "AIC") %>%
  ggplot()+
  geom_freqpoly(aes(x = AIC), bins = 30) +
  geom_vline(xintercept = mod_vMF$AIC, col = "blue") +
  geom_rug(aes(x = AIC))
```

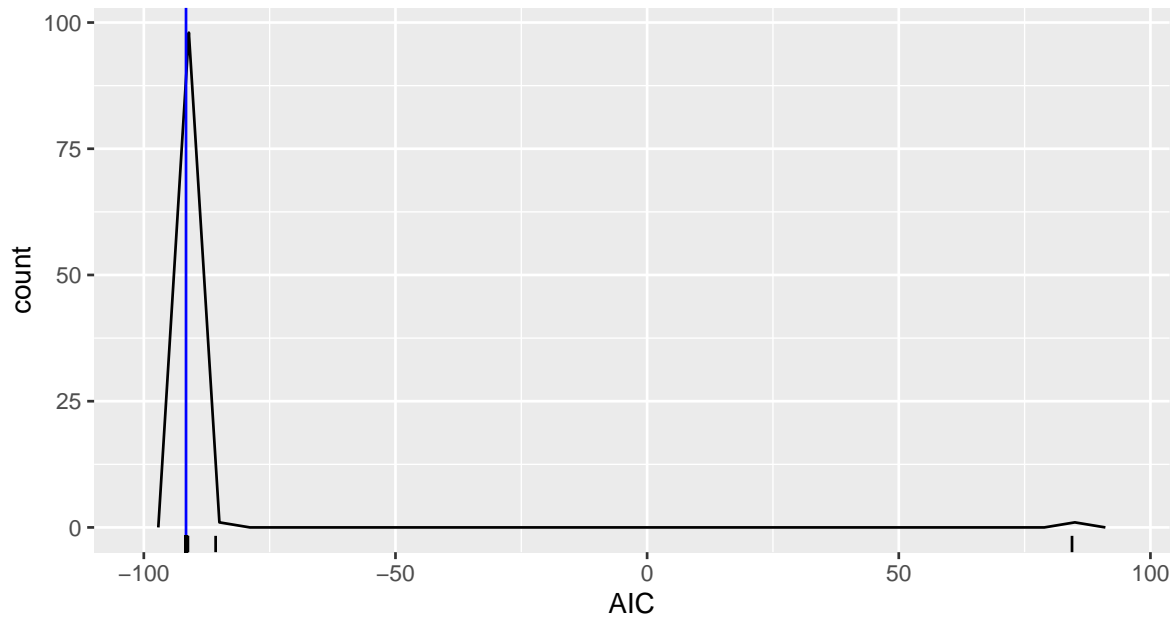

```
idx <- which.min(lapply(mod_vMF_restarts, "[", "AIC") %>% unlist())
mod_vMF <- mod_vMF_restarts[[idx]]
mod_vMF$k
```

```
[1] 38.64599
```

```
mod_vMF$AIC
```

```
[1] -91.61656
```

Below is plot for comparing likelihoods for give simulated response y.

```
getlikR <- function(y){
  mod1 <- mobius_vMF(y,
    xs = NULL,
    xe = mod_vMF$xe,
    type = "LinEuc",
    start = mod_vMF$est)
  mod2 <- withCallingHandlers({mobius_SvMF(y,
    xs = NULL,
    xe = mod_vMF$xe,
    type = "LinEuc",
```



```

        G01behaviour = "free",
        mean = mod_SvMF$mean,
        k = mod_SvMF$k,
        a = mod_SvMF$a,
        G0 = mod_SvMF$G0)},
    warning = function(w){
      if (grepl("p!=3", conditionMessage(w))) {
        invokeRestart("muffleWarning")
      }
    })
  if ((mod1$nlOPT$status != 4) || (mod2$nlOPT$status != 4)){
    return(list(likR = NA_real_,
      vMF = mod1,
      SvMF = mod2))
  }
  lLik1 <- ldMobius_SvMF(mod1$y, xs = NULL, xe =mod1$xe,
    mean = mod1$est,
    k = mod1$k,
    a = rep(1, 5),
    G0 = mod2$G0) %>%
    colSums()
  lLik2 <- ldMobius_SvMF(mod2$y, xs = NULL, xe =mod2$xe,
    mean = mod2$mean,
    k = mod2$k,
    a = mod2$a,
    G0 = mod2$G0) %>%
    colSums()

  list(likR = -2* (lLik1[["R"]] - lLik2[["R"]]),
    vMF = mod1,
    SvMF = mod2)
}

```

Now we simulate the response 1000 times from the best vMF model and compare the likelihood of the vMF model to the likelihood of the SvMF model on each simulated data.

```

null_likRs <- pbapply::pblapply(1:1000, function(seed){
  set.seed(seed)
  y_ld <- rMobius_SvMF(xs = NULL,
    xe = mod_vMF$xe,
    mean = mod_vMF$mean,
    k = mod_vMF$k,

```

```

a = rep(1, 5),
G0 = diag(1,5))
sum(y_ld[,6])
y <- y_ld[,-6]
getlikR(y)
})

```

Warning in optim\_constV(y, xs, xe, mean = preest\$mean, k = if (!is.null(k)) {:  
NLOPT\_MAXEVAL\_REACHED: Optimization stopped because maxeval (above) was  
reached.

Warning in mobius\_vMF(y, xs = NULL, xe = mod\_vMF\$xe, type = "LinEuc", start =  
mod\_vMF\$est): NLOPT\_MAXEVAL\_REACHED: Optimization stopped because maxeval  
(above) was reached.

Warning in optim\_constV(y, xs, xe, mean = preest\$mean, k = if (!is.null(k)) {:  
NLOPT\_MAXEVAL\_REACHED: Optimization stopped because maxeval (above) was  
reached.

Warning in optim\_constV(y, xs, xe, mean = preest\$mean, k = if (!is.null(k)) {:  
NLOPT\_MAXEVAL\_REACHED: Optimization stopped because maxeval (above) was  
reached.

Warning in mobius\_vMF(y = y, xs = xs, xe = xe, start = mean, type = type, :  
NLOPT\_MAXEVAL\_REACHED: Optimization stopped because maxeval (above) was  
reached.

Warning in optim\_constV(y, xs, xe, mean = preest\$mean, k = if (!is.null(k)) {:  
NLOPT\_MAXEVAL\_REACHED: Optimization stopped because maxeval (above) was  
reached.

Warning in optim\_constV(y, xs, xe, mean = preest\$mean, k = if (!is.null(k)) {:  
NLOPT\_MAXEVAL\_REACHED: Optimization stopped because maxeval (above) was  
reached.

```

obs <- getlikR(s4df_clean %>%
  select(s1, s2, sMrt, sMrf, sMtf) %>%
  st_drop_geometry() %>%
  as.matrix())

```

```
null_likRs_vec <- lapply(null_likRs, "[", "likR") %>% unlist()
sum(is.na(null_likRs_vec))
```

```
[1] 6
```

```
sum(!is.na(null_likRs_vec))
```

```
[1] 994
```

There were a few cases where the regression did not converge, and these have been discarded.  $p$ -value is the probability, under the null, of getting a likelihood-ratio that is at least as large as the observed ratio:

```
mean(null_likRs_vec > obs$likR, na.rm = TRUE)
```

```
[1] 0.002012072
```

This small  $p$ -value suggests that the data was not drawn from a vMF regression.

## 11 Parametric Bootstrap Regions for a

Lets look at the CI for the scales of the SvMF. We do this by simulating from the fitted SvMF model 1000 times, and refitting a SvMF regression each time.

```
Bests <- pbapply::pblapply(1:1000, function(seed){
  set.seed(seed)
  y <- rMobius_SvMF(xs = NULL,
    xe = mod_SvMF$xe,
    mean = mod_SvMF$mean,
    k = mod_SvMF$k,
    a = mod_SvMF$a,
    G0 = mod_SvMF$G0)[,-6]
  newmod <- withCallingHandlers({mobius_SvMF(y,
    xs = NULL,
    xe = mod_SvMF$xe,
    type = "LinEuc",
    G0behaviour = "free",
    mean = mod_SvMF$mean,
```

```

      k = mod_SvMF$k,
      a = mod_SvMF$a,
      G0 = mod_SvMF$G0}},
  warning = function(w){
    if (grepl("p!=3", conditionMessage(w))) {
      invokeRestart("muffleWarning")
    }
  })
  return(newmod[c("mean", "k", "a", "G0")])
}, cl = 2)

```

```

Bests_a <- lapply(Bests, "[", "a") %>%
  simplify2array() %>%
  t()
colnames(Bests_a) <- paste0("a", 1:5)
summary(Bests_a)

```

|          | a1 | a2            | a3             | a4             | a5             |
|----------|----|---------------|----------------|----------------|----------------|
| Min.     | :1 | Min. :1.718   | Min. :0.9883   | Min. :0.6278   | Min. :0.1288   |
| 1st Qu.: | :1 | 1st Qu.:2.266 | 1st Qu.:1.3975 | 1st Qu.:0.9007 | 1st Qu.:0.2406 |
| Median : | :1 | Median :2.458 | Median :1.5239 | Median :0.9869 | Median :0.2743 |
| Mean :   | :1 | Mean :2.467   | Mean :1.5329   | Mean :0.9951   | Mean :0.2777   |
| 3rd Qu.: | :1 | 3rd Qu.:2.656 | 3rd Qu.:1.6568 | 3rd Qu.:1.0797 | 3rd Qu.:0.3073 |
| Max.     | :1 | Max. :3.414   | Max. :2.5347   | Max. :1.5542   | Max. :0.6289   |

## 11.1 95% CI for a (SI Table)

```

df <- rbind(mod_SvMF$a[-1],
            apply(Bests_a[-1], 2, quantile, probs = c(0.025, 0.975)) %>%
              round(2)) %>%
  as.data.frame()
row.names(df) <- c("Estimate", "Lower", "Upper")
mykbl <- df %>%
  mutate(across(everything(), ~formatC(.x, digits = 2, format = "f"))) %>%
  kbl(booktabs = TRUE, position = "!h", escape = FALSE, format = "latex",
      col.names = paste0("a", 2:5)) %>%
  add_header_above(c(" "=1, "Scales" = 4), escape = FALSE)
mykbl

```

|          | Scales |      |      |      |
|----------|--------|------|------|------|
|          | a2     | a3   | a4   | a5   |
| Estimate | 2.08   | 1.40 | 1.00 | 0.34 |
| Lower    | 1.95   | 1.17 | 0.75 | 0.19 |
| Upper    | 3.04   | 1.94 | 1.31 | 0.40 |
